# Supplementary material for: Warm-starting DARTS using meta-learning
Source: arXiv:2205.06355 source file (2022-05-12)
Supplement: Supplementary file 1 [file 06_appendix.tex]

\section*{Appendix A. Discovered transfer architectures}
\label{app:a}

\begin{sidewaysfigure}[!h]
    \centering
    \begin{subfigure}[b]{1\textwidth}
        \includegraphics[width=1\linewidth]{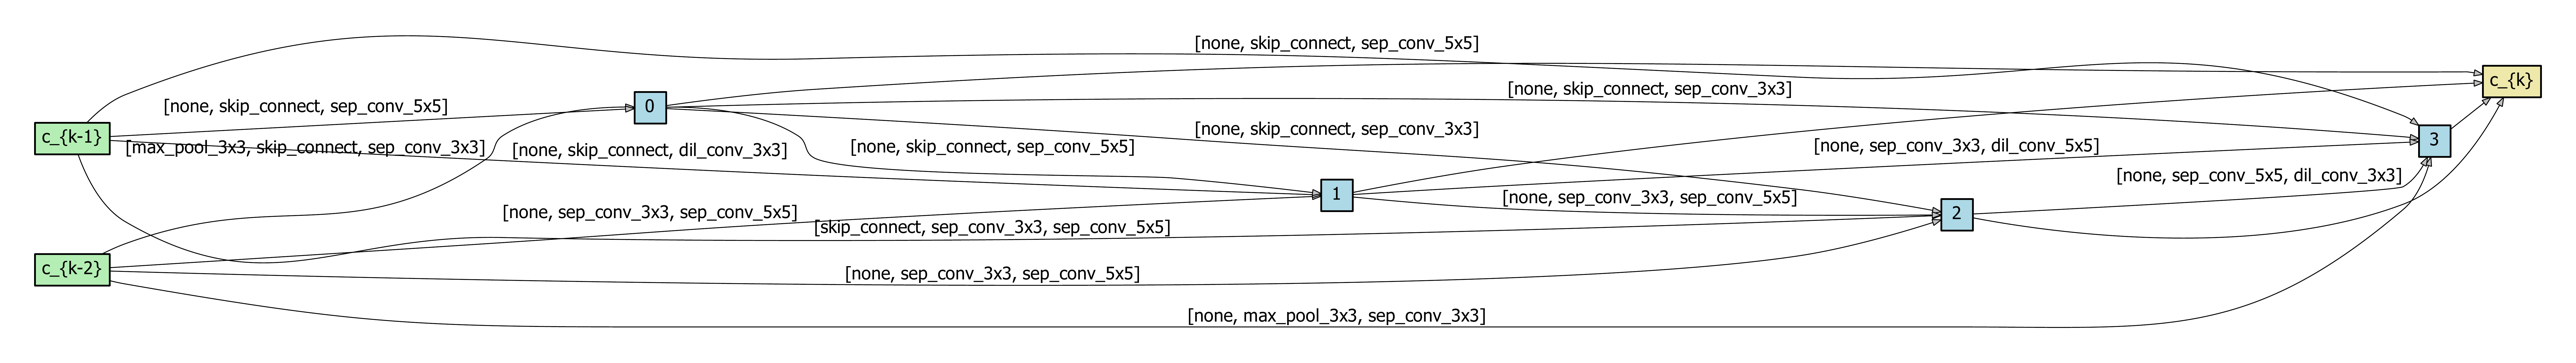}
        \caption{Normal cell found on \textit{dtd} task}
   \label{fig:Ng1} 
    \end{subfigure}
    \begin{subfigure}[b]{1\textwidth}
\includegraphics[width=1\linewidth]{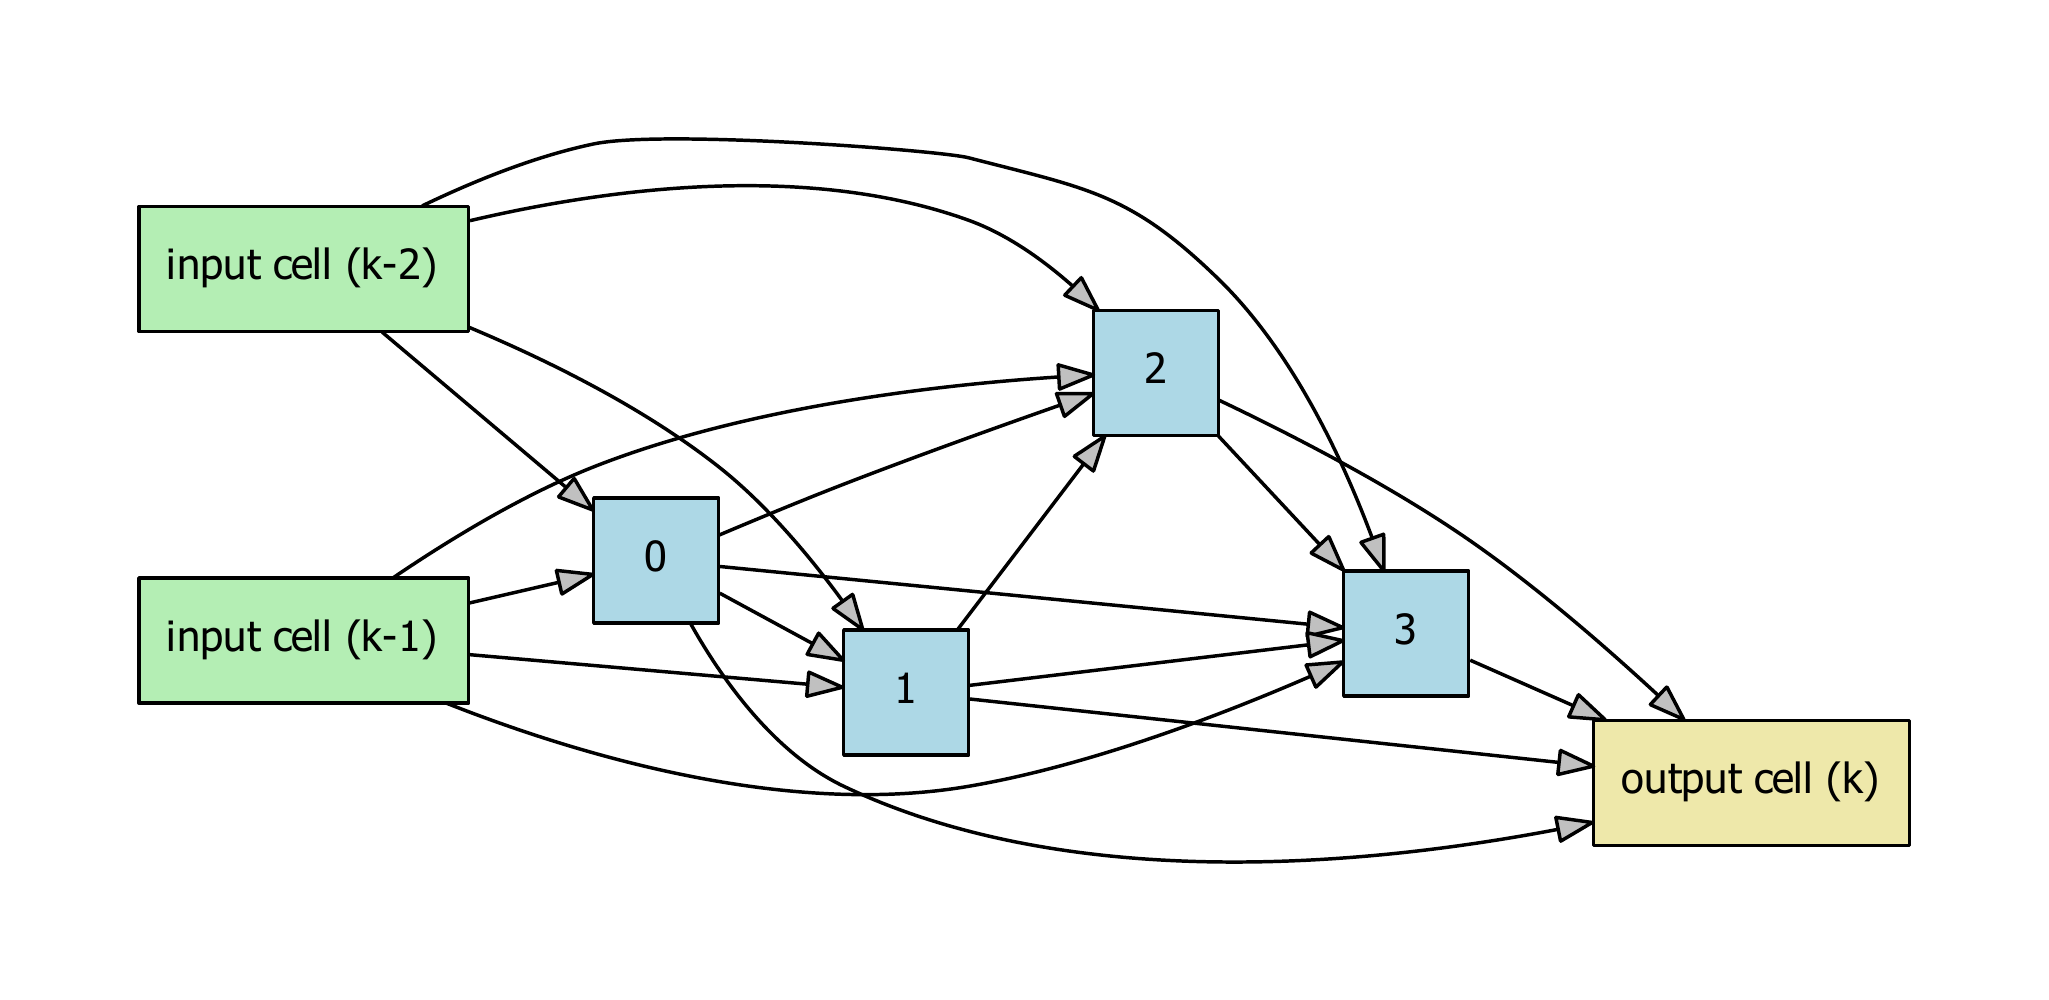}
        \caption{Reduction cell found on \textit{aircraft} task}
   \label{fig:Ng2}
    \end{subfigure}
    \caption{Abstract illustration of Neural Architecture.}
    \label{fig:search-space}
\end{sidewaysfigure}

\section*{Appendix B. Discover architectures by warm-starting DARTS using transfer architecture}
\label{app:b}

\begin{figure}[!h]
    \centering
    \begin{subfigure}[b]{0.49\textwidth}
        \includegraphics[width=1\linewidth]{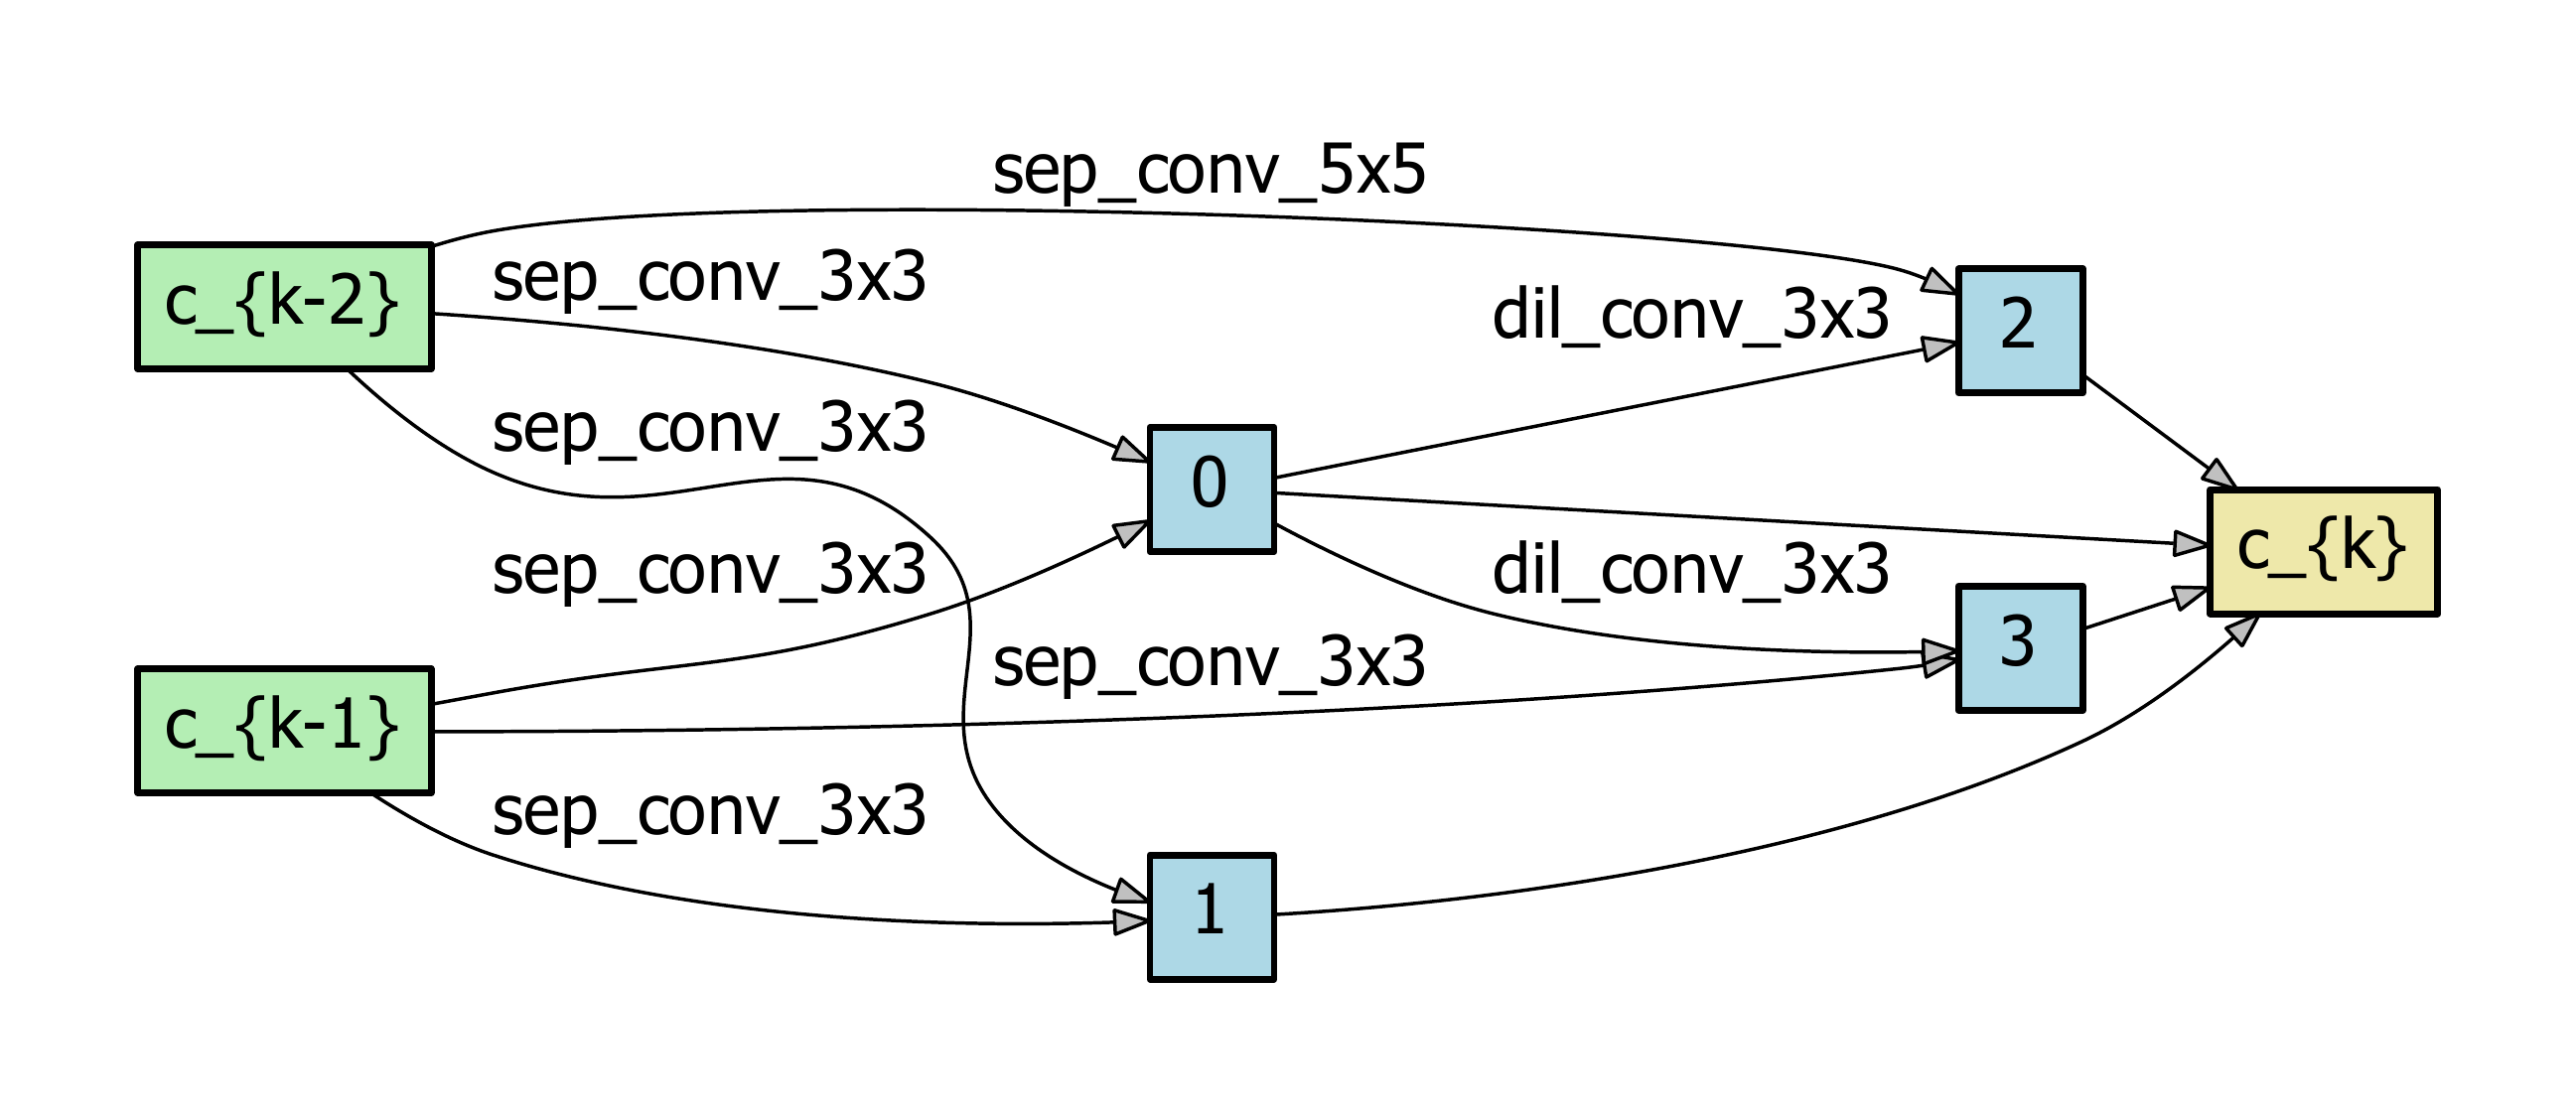}
        \caption{Normal cell found on \textit{aircraft} task}
   \label{fig:Ng1} 
    \end{subfigure}
    \begin{subfigure}[b]{0.49\textwidth}
\includegraphics[width=1\linewidth]{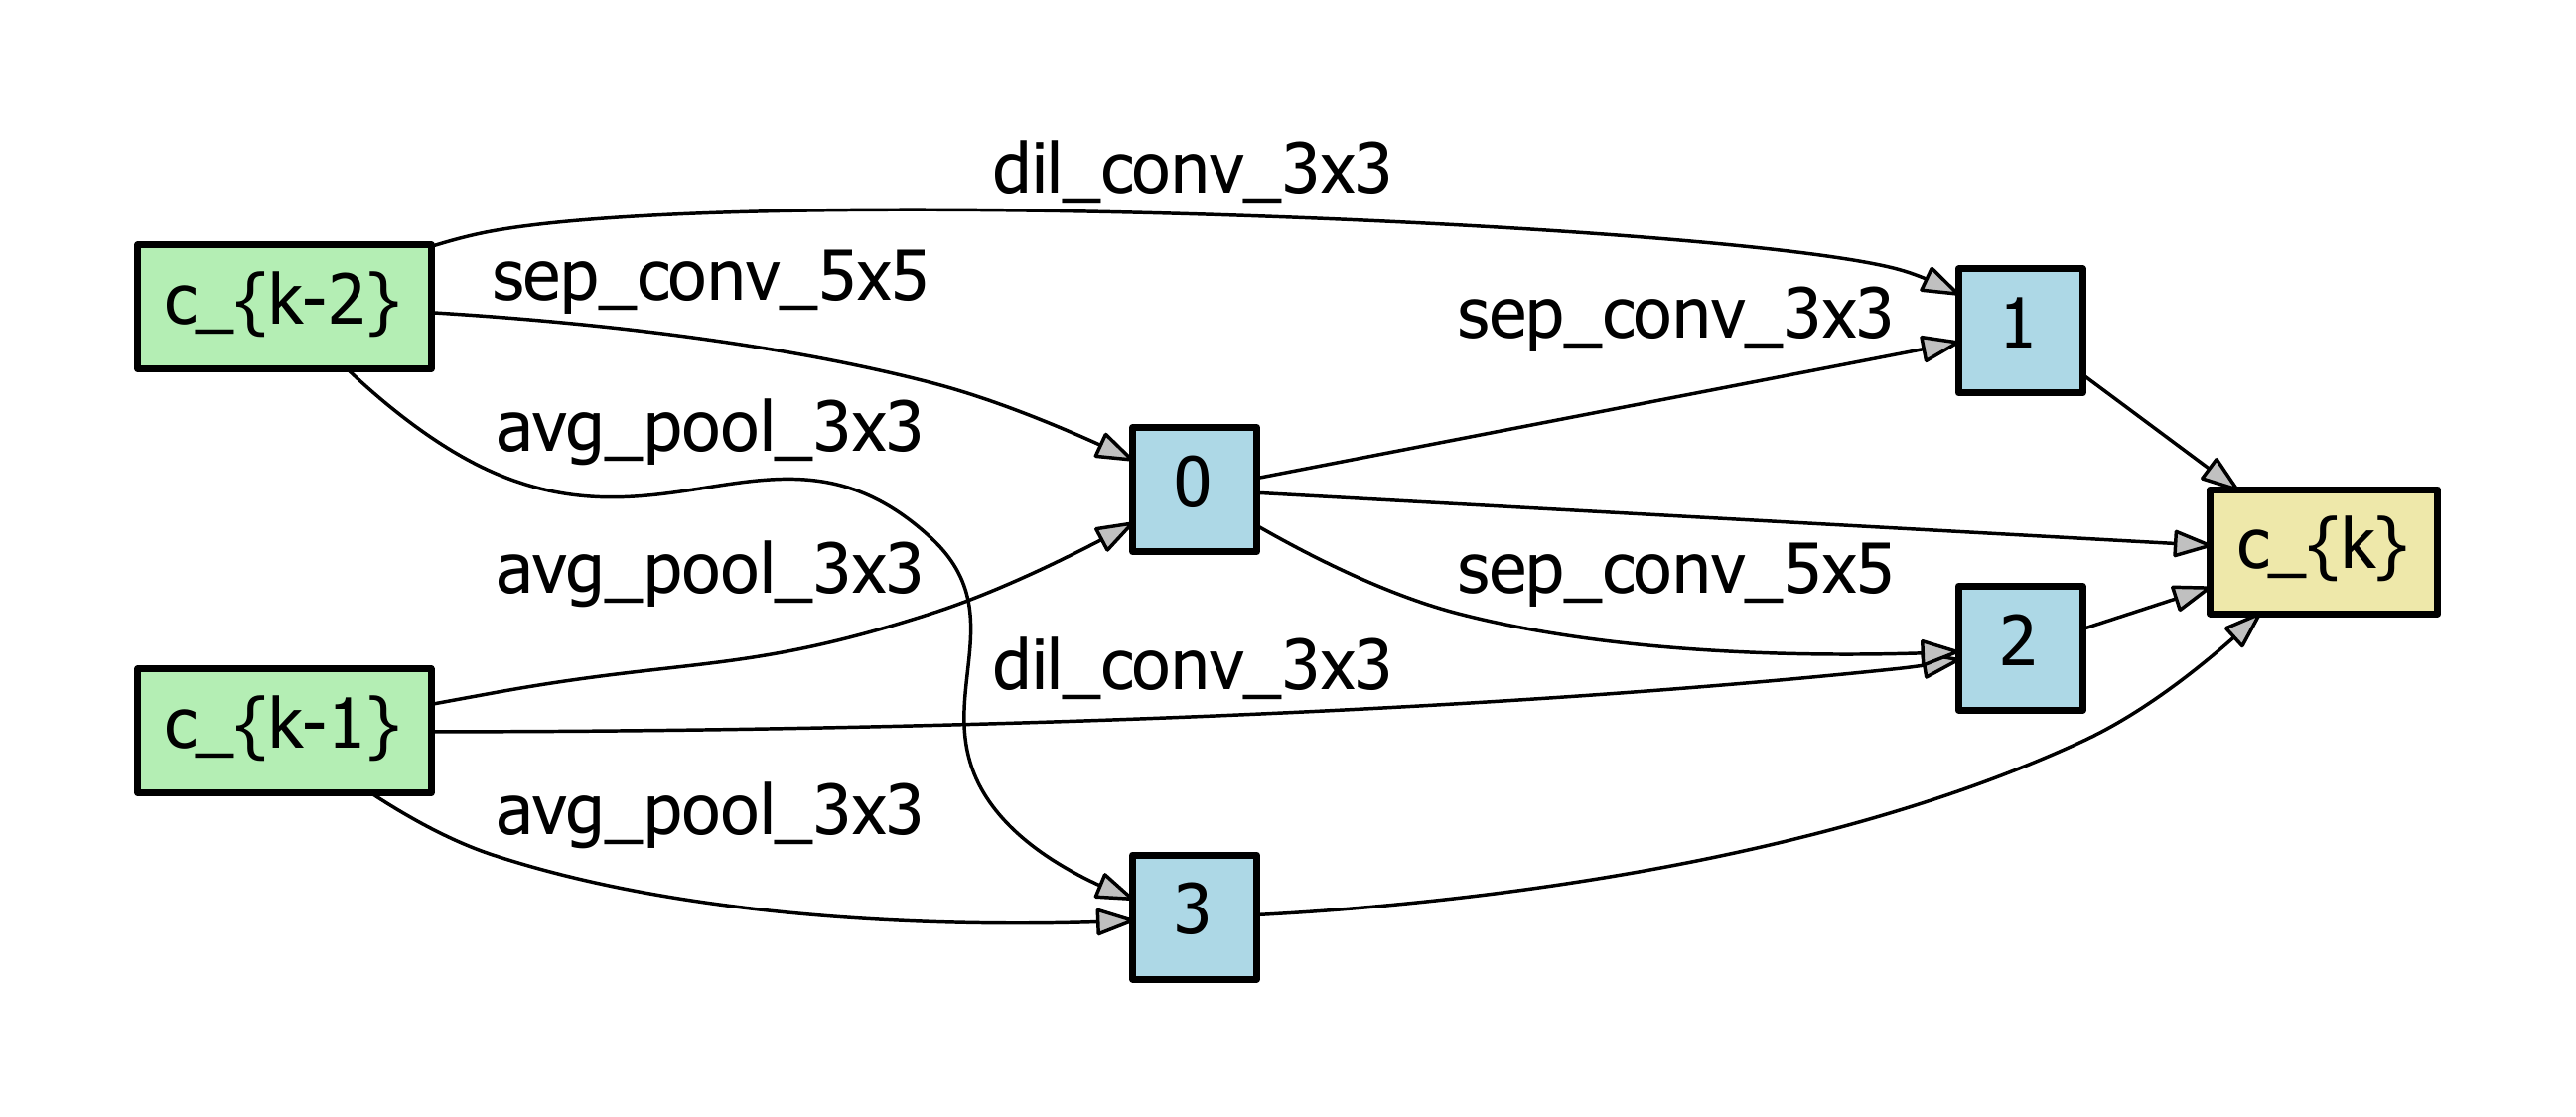}
        \caption{Reduction cell found on \textit{aircraft} task}
   \label{fig:Ng2}
    \end{subfigure}
    \begin{subfigure}[b]{0.49\textwidth}
        \includegraphics[width=1\linewidth]{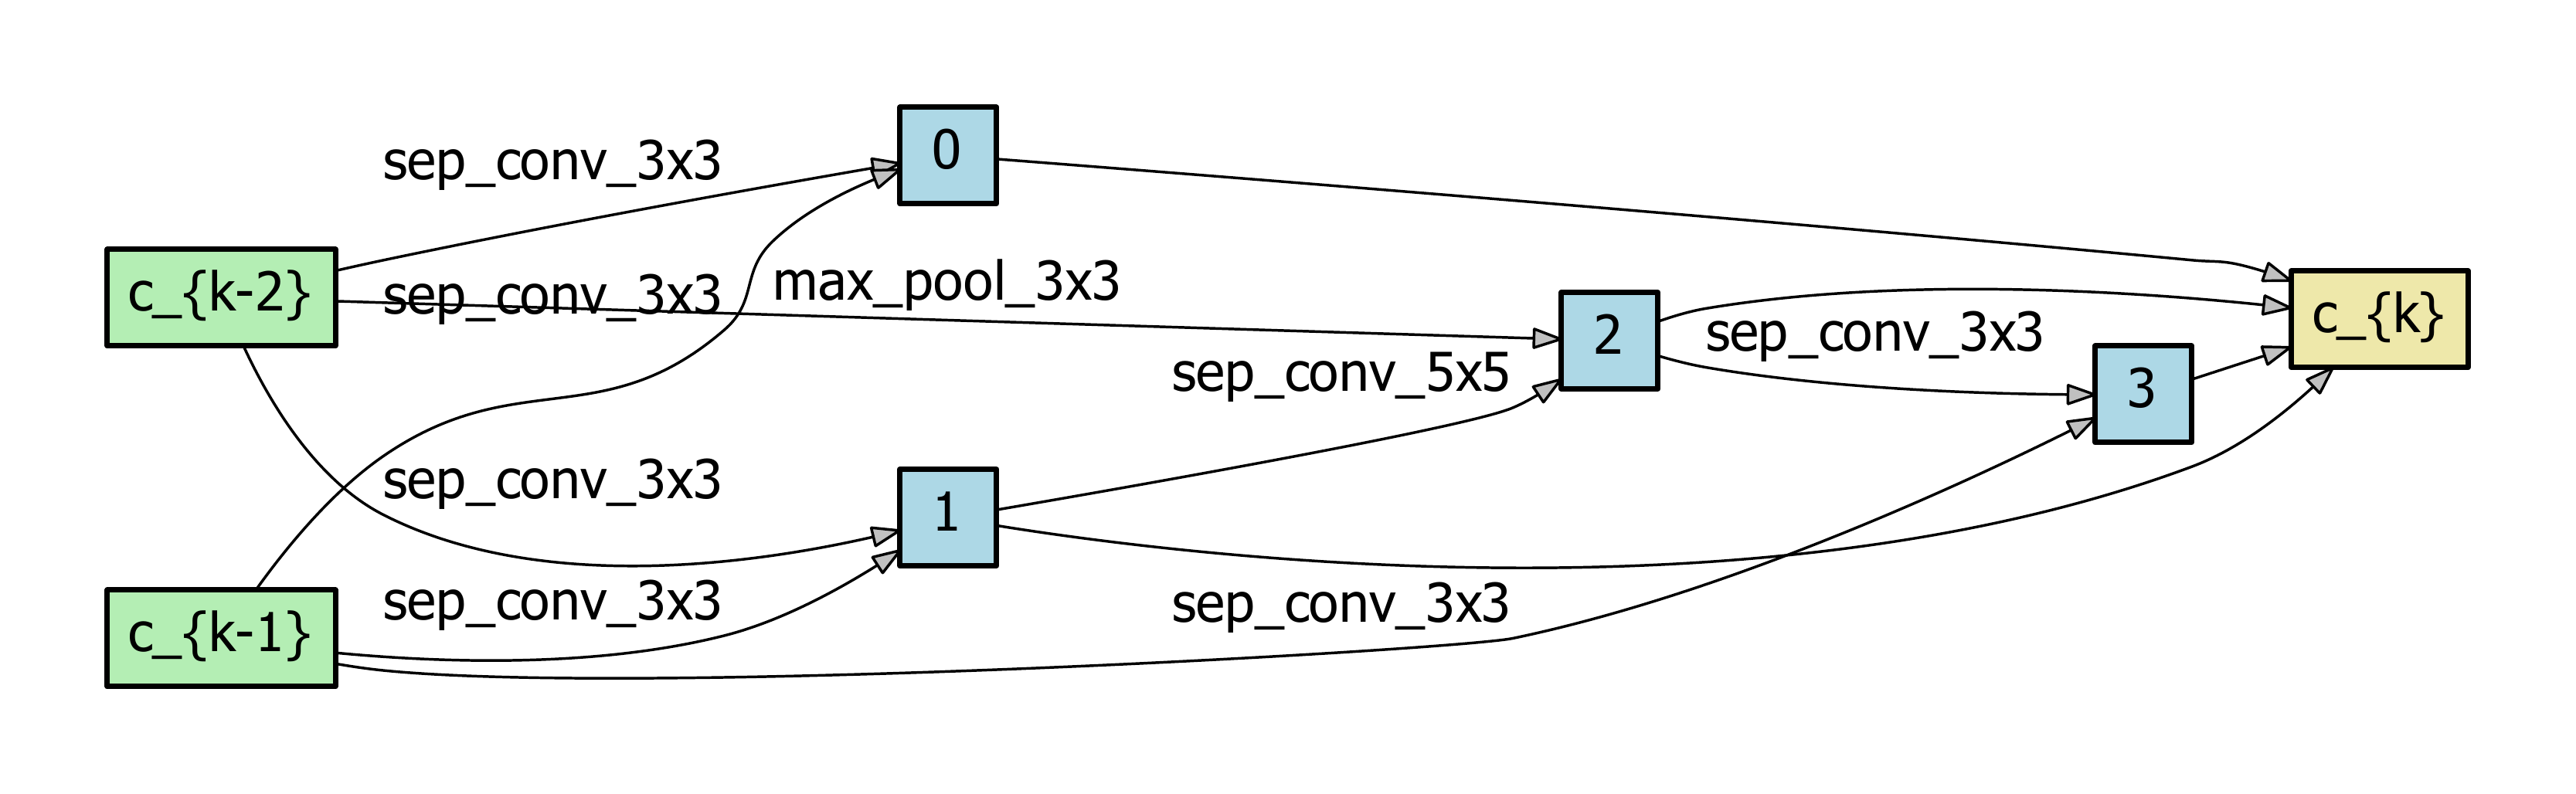}
        \caption{Normal cell found on \textit{dtd} task}
   \label{fig:Ng1} 
    \end{subfigure}
    \begin{subfigure}[b]{0.49\textwidth}
\includegraphics[width=1\linewidth]{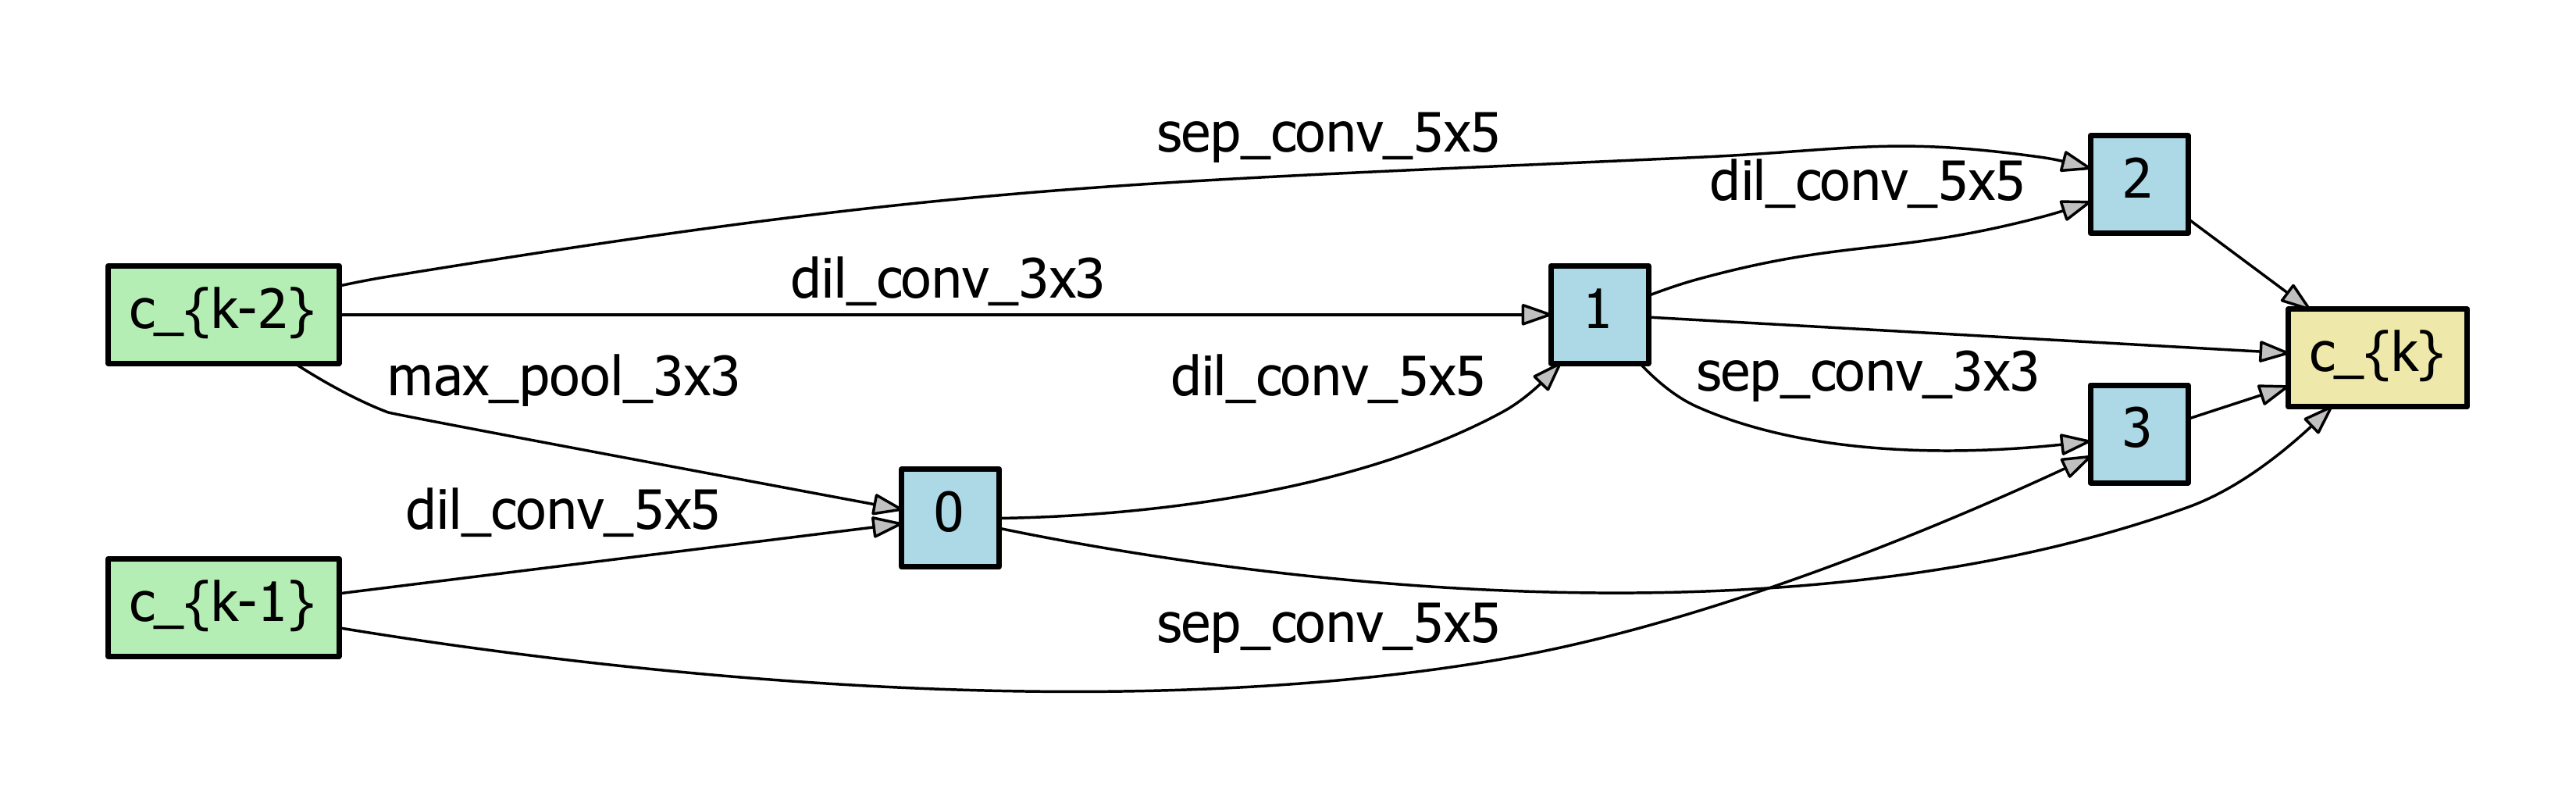}
        \caption{Reduction cell found on \textit{aircraft} task}
   \label{fig:Ng2}
    \end{subfigure}
    \caption{Abstract illustration of Neural Architecture Search methods \cite{elsken2019survey}.}
    \label{fig:search-space}
\end{figure}

\begin{figure}[h]
    \centering
    \begin{subfigure}[b]{0.49\textwidth}
        \includegraphics[width=1\linewidth]{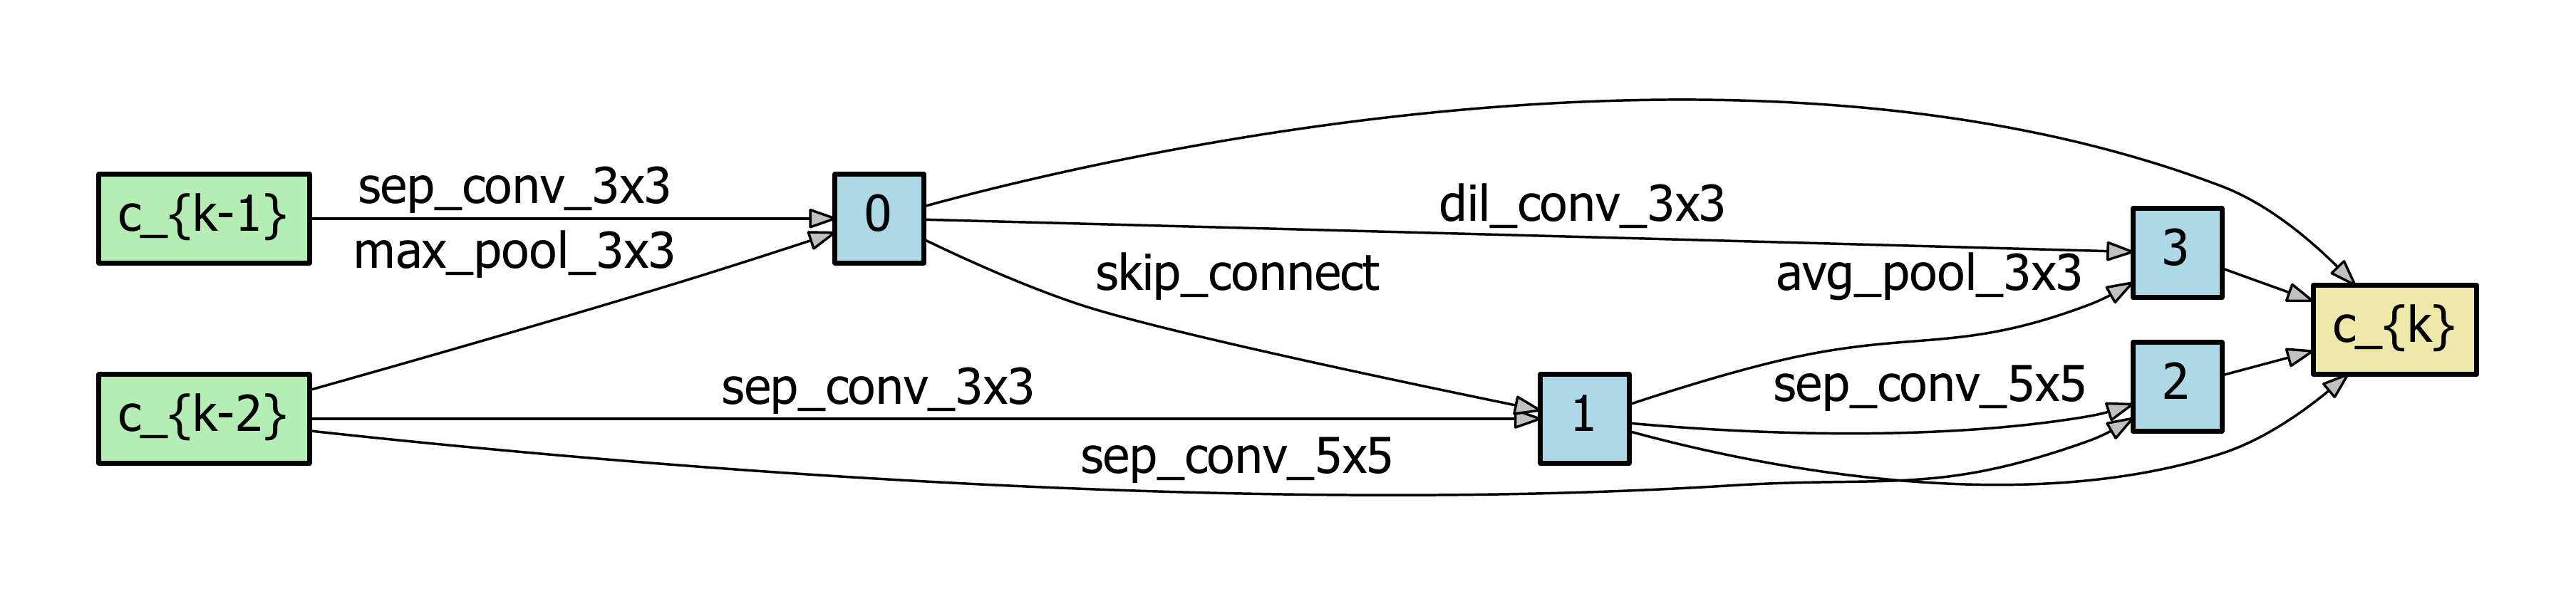}
        \caption{Normal cell found on \textit{flower} task}
   \label{fig:Ng1} 
    \end{subfigure}
    \begin{subfigure}[b]{0.49\textwidth}
\includegraphics[width=1\linewidth]{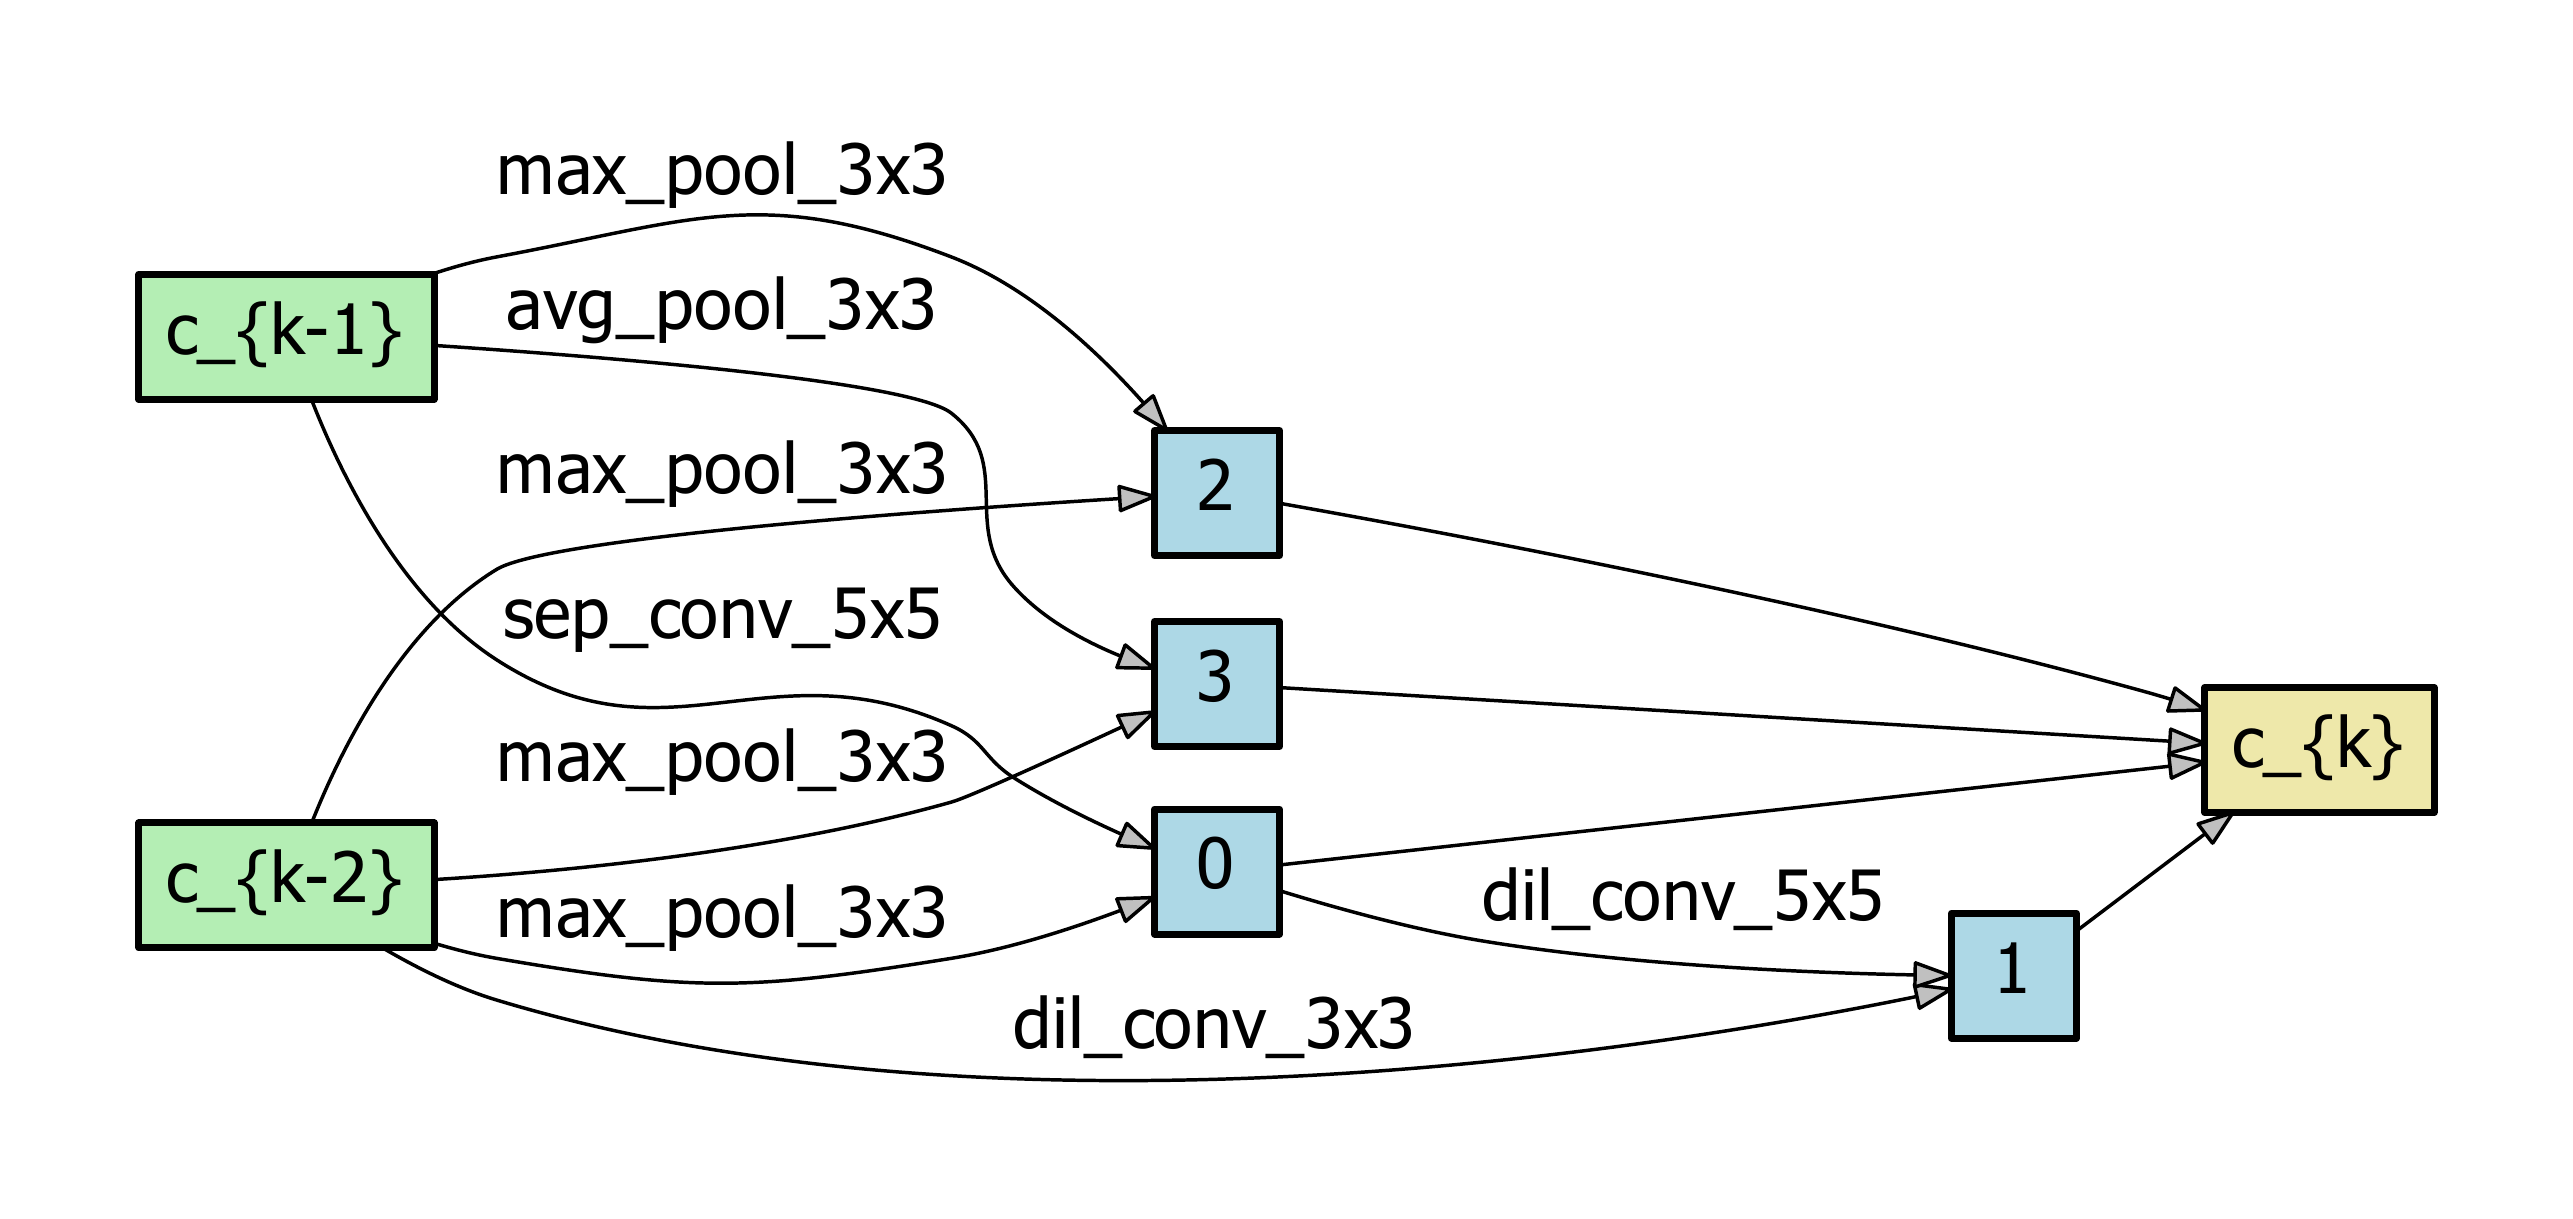}
        \caption{Reduction cell found on \textit{flower} task}
   \label{fig:Ng2}
    \end{subfigure}
    \begin{subfigure}[b]{0.49\textwidth}
        \includegraphics[width=1\linewidth]{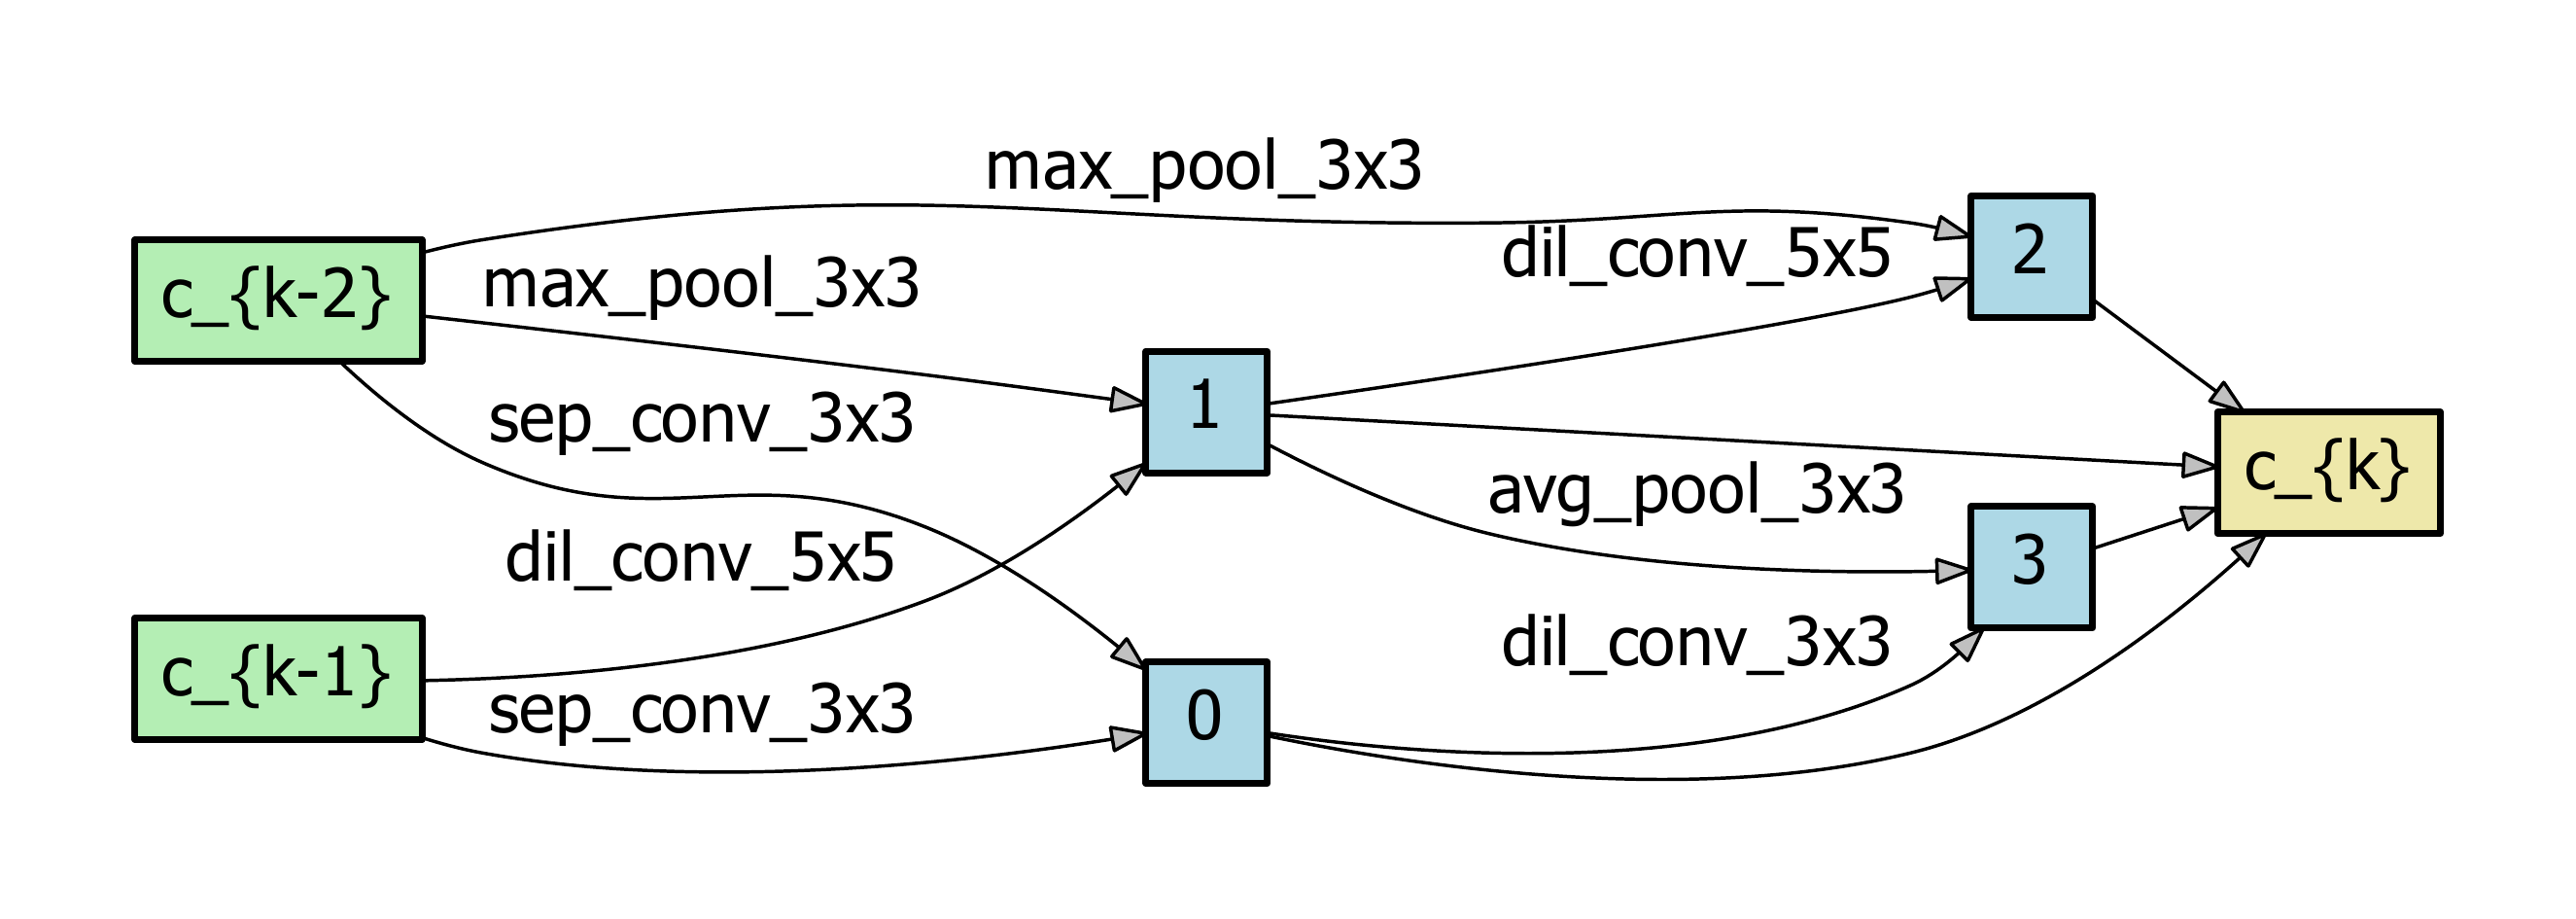}
        \caption{Normal cell found on \textit{flower} task}
   \label{fig:Ng1} 
    \end{subfigure}
    \begin{subfigure}[b]{0.49\textwidth}
\includegraphics[width=1\linewidth]{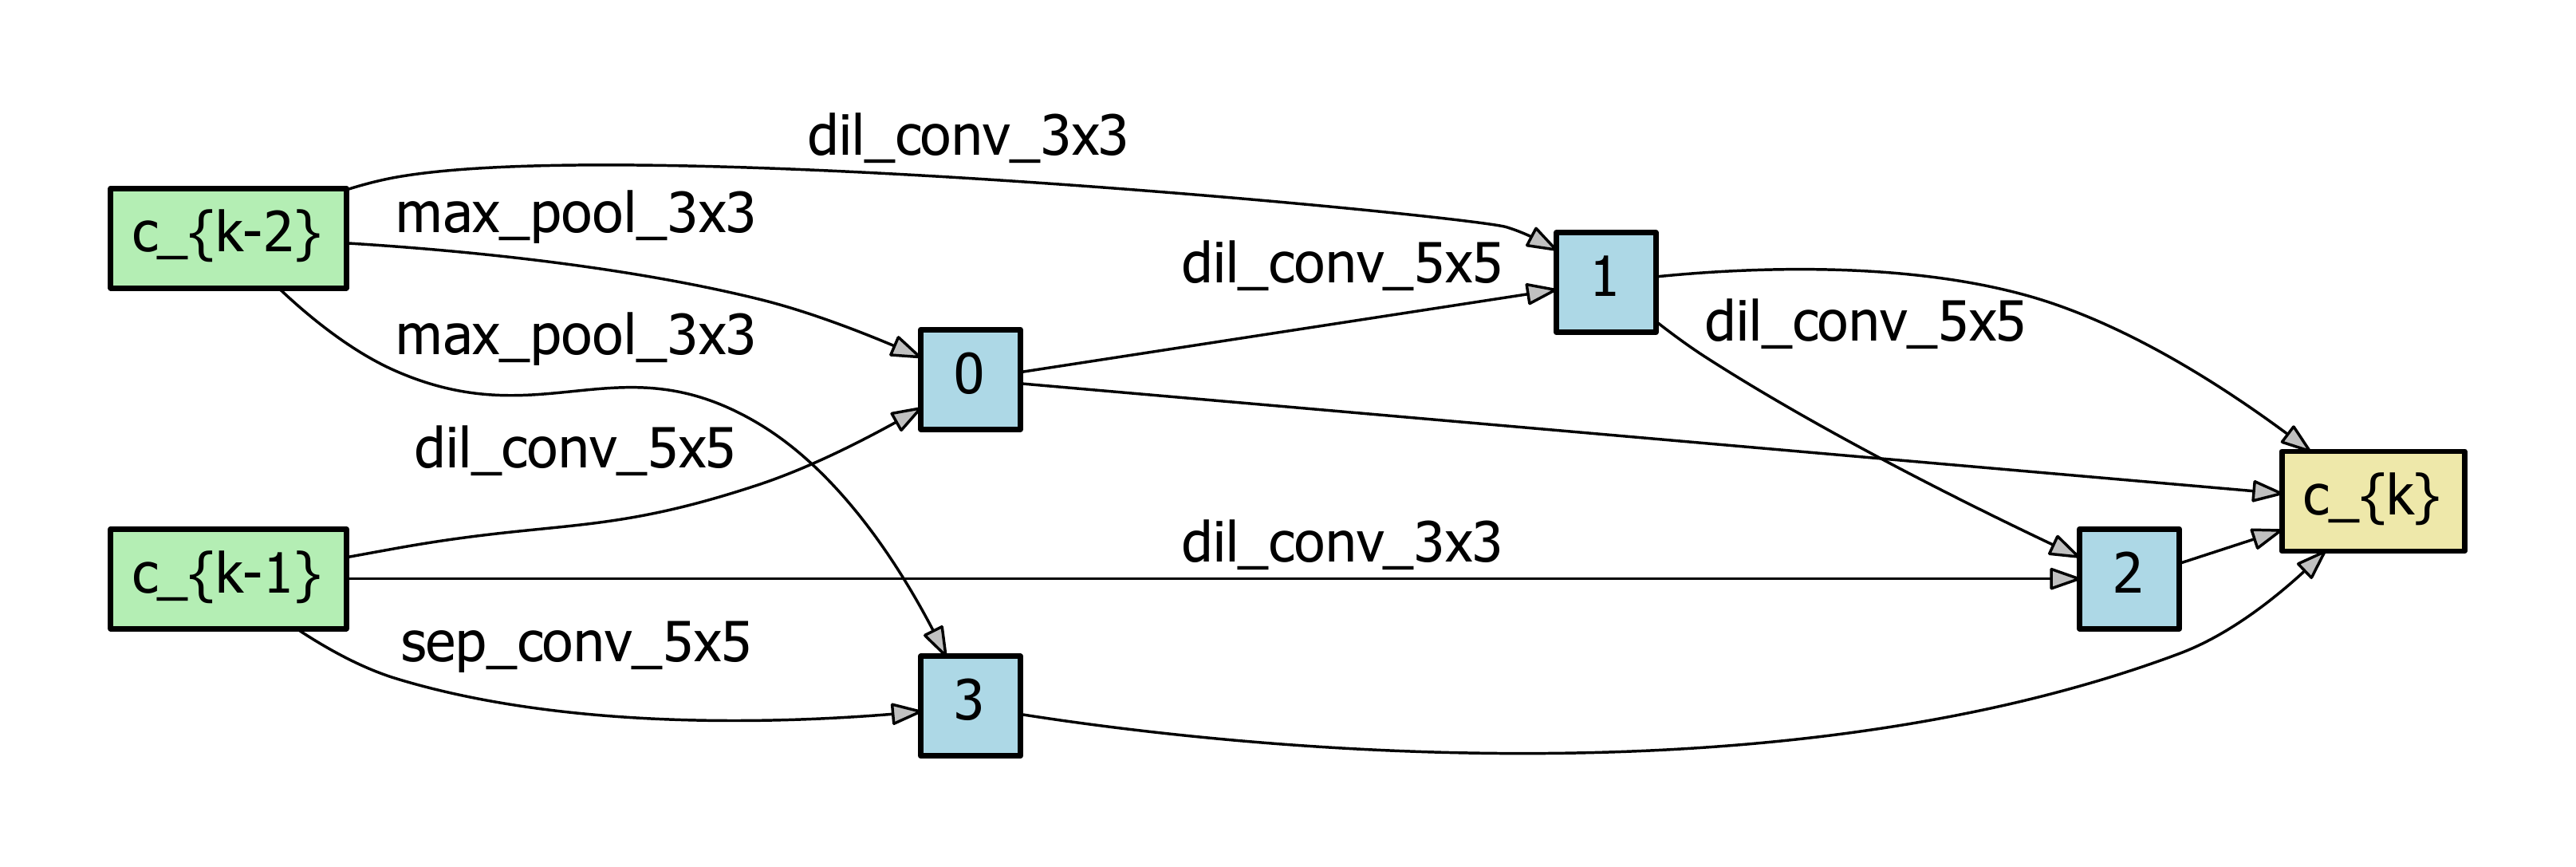}
        \caption{Reduction cell found on \textit{flower} task}
   \label{fig:Ng2}
    \end{subfigure}
    \caption{Abstract illustration of Neural Architecture Search methods \cite{elsken2019survey}.}
    \label{fig:search-space}
\end{figure}

\begin{figure}[]
    \centering
    \begin{subfigure}[b]{0.49\textwidth}
        \includegraphics[width=1\linewidth]{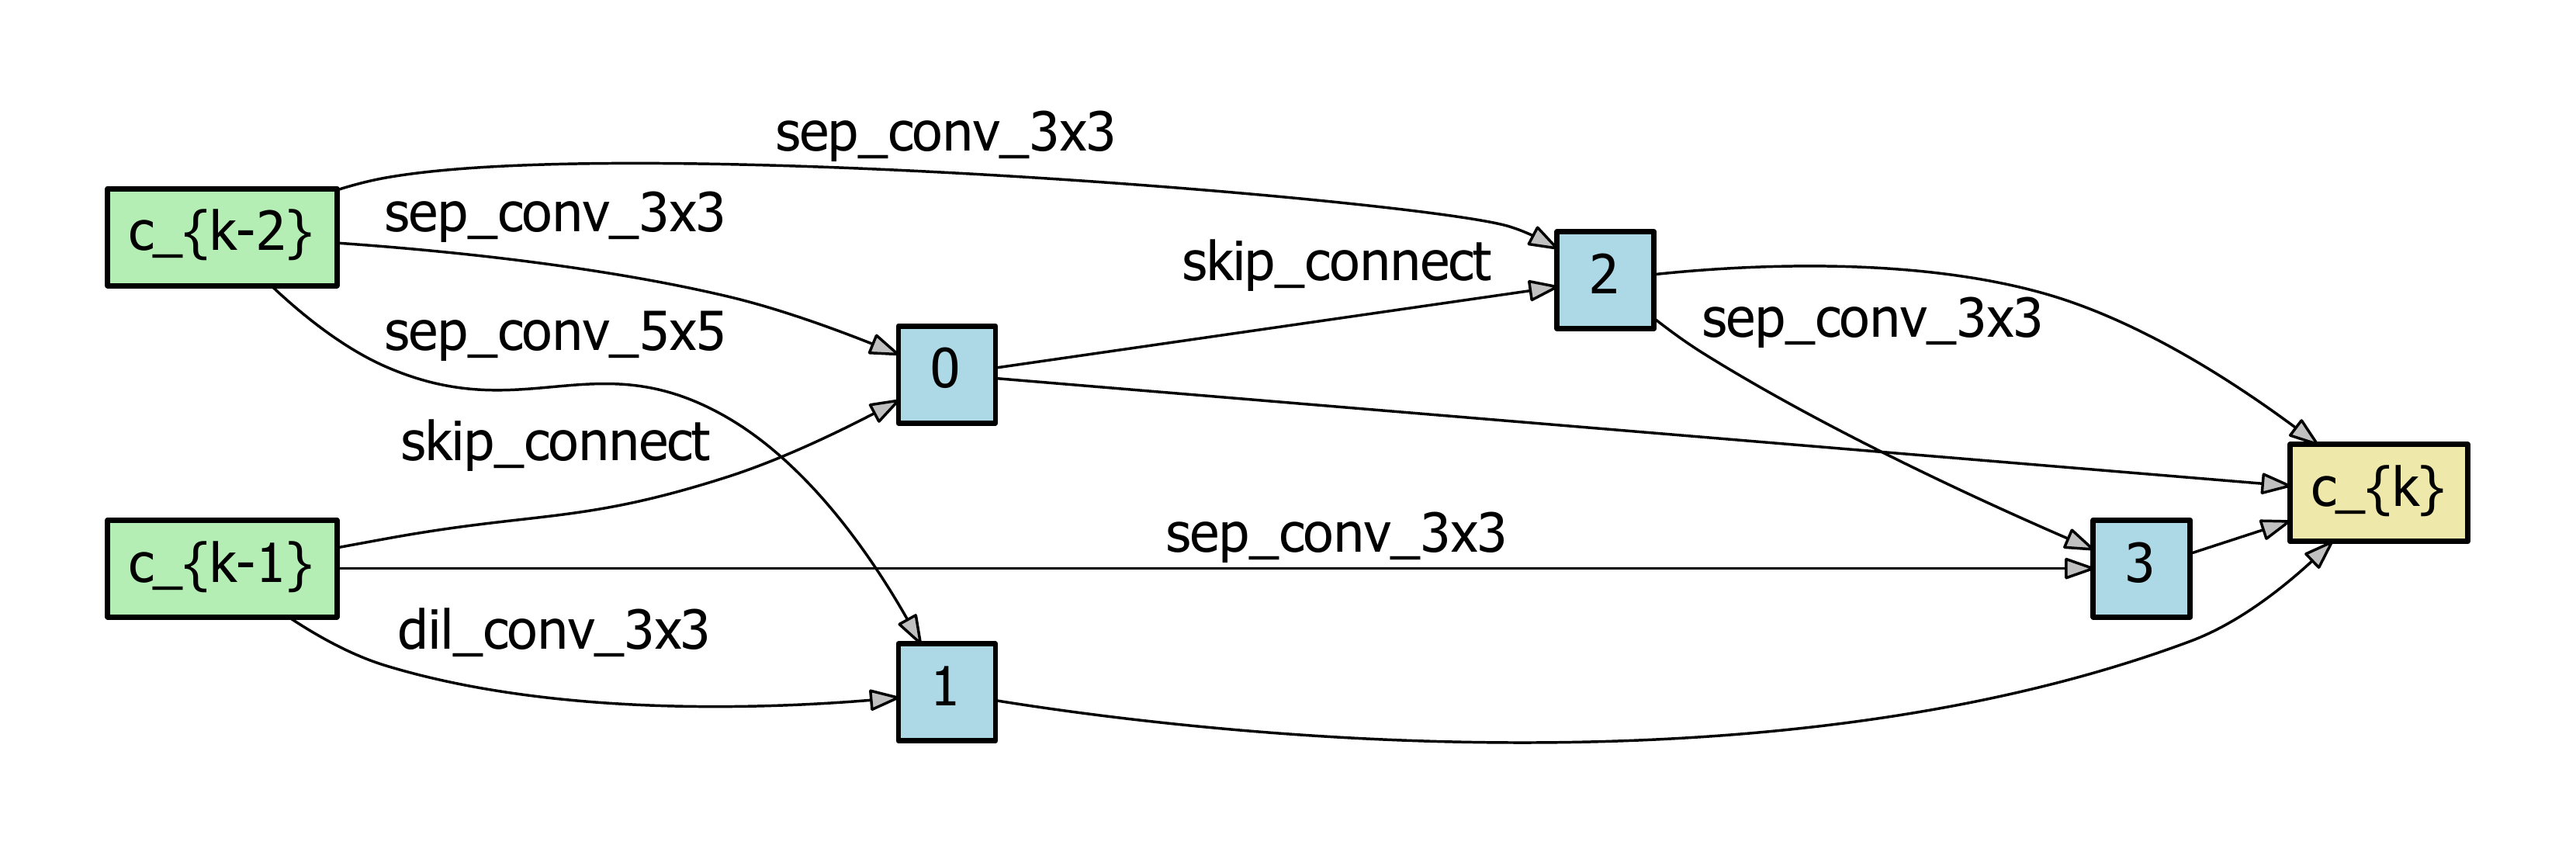}
        \caption{Normal cell found on \textit{flower} task}
   \label{fig:Ng1} 
    \end{subfigure}
    \begin{subfigure}[b]{0.49\textwidth}
\includegraphics[width=1\linewidth]{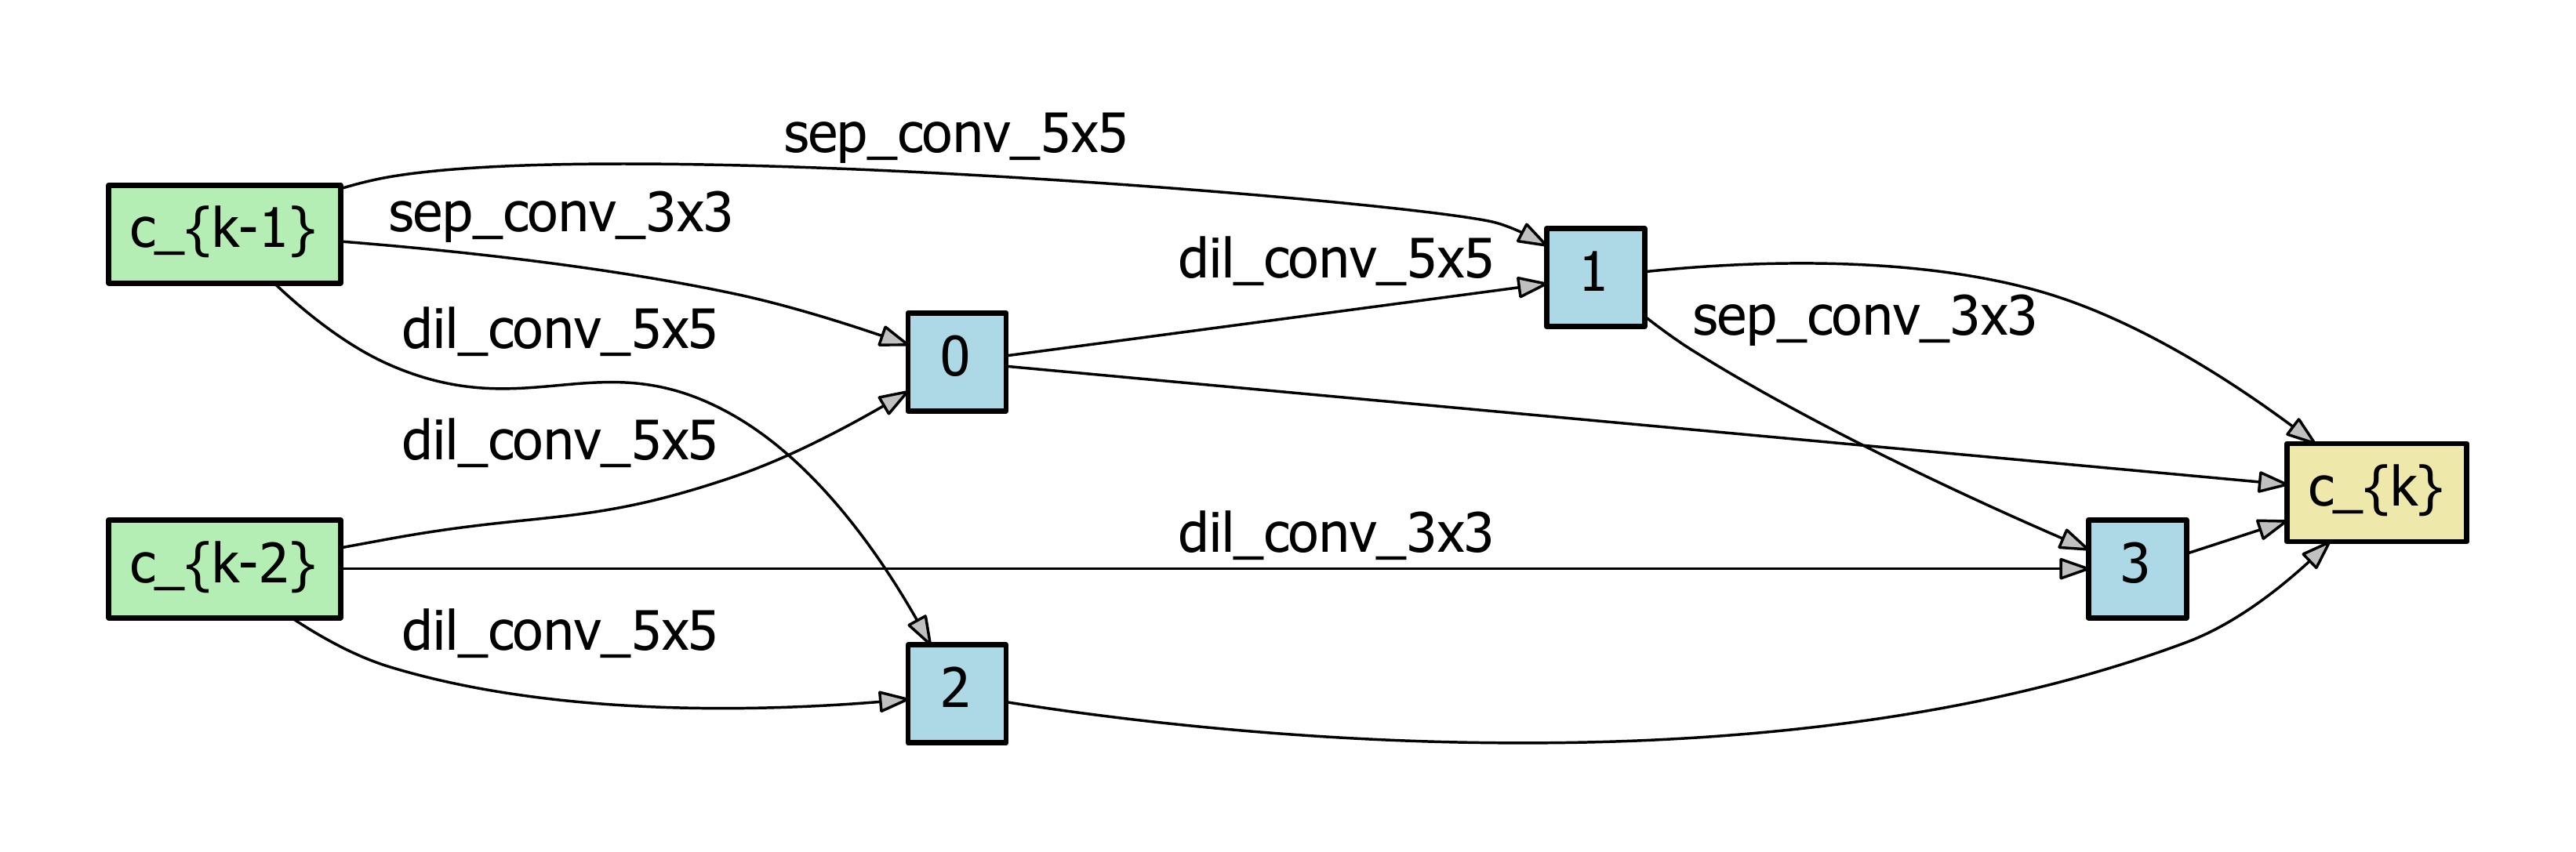}
        \caption{Reduction cell found on \textit{flower} task}
   \label{fig:Ng2}
    \end{subfigure}
    \begin{subfigure}[b]{0.49\textwidth}
        \includegraphics[width=1\linewidth]{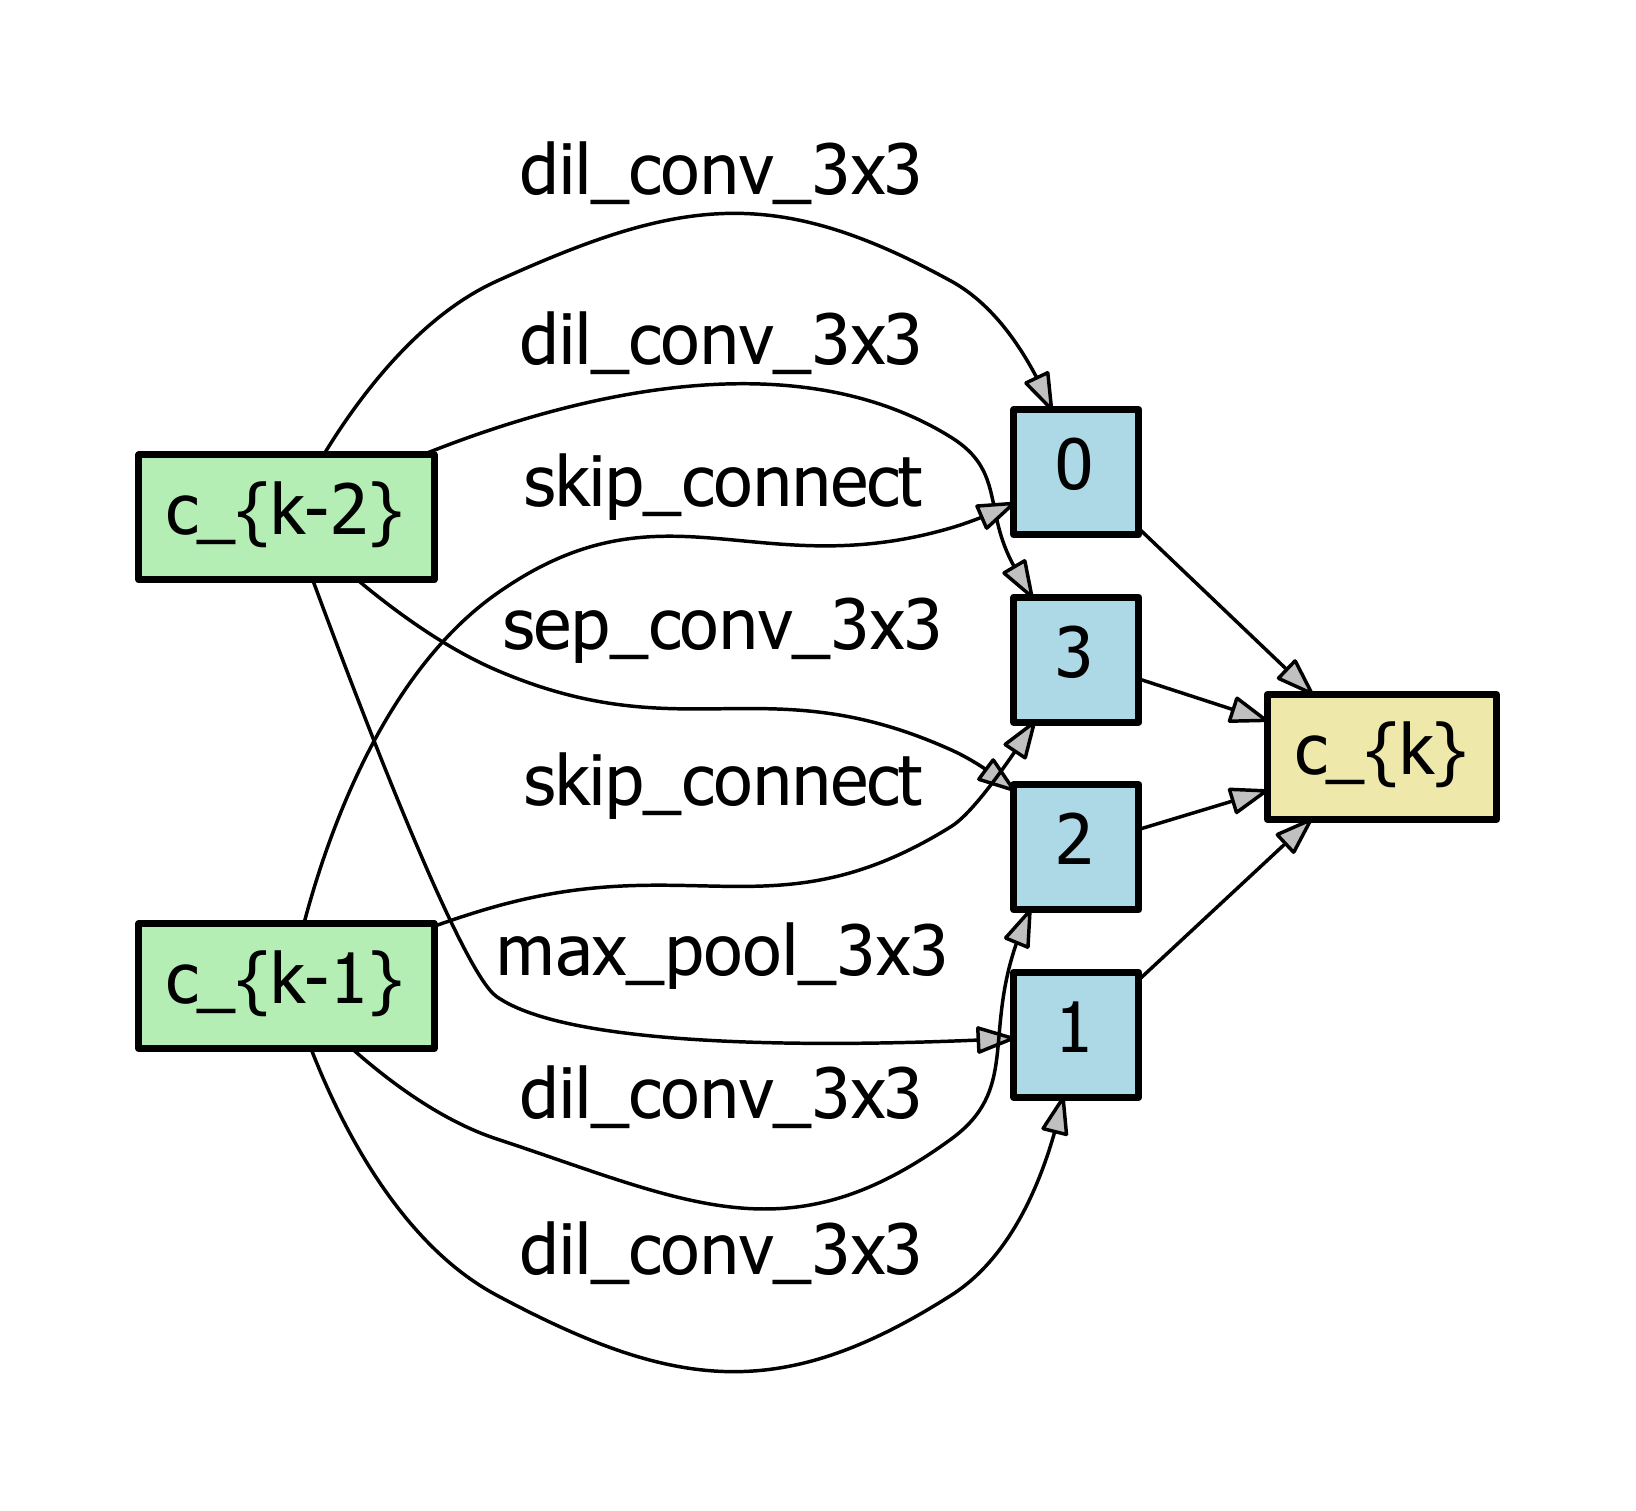}
        \caption{Normal cell found on \textit{flower} task}
   \label{fig:Ng1} 
    \end{subfigure}
    \begin{subfigure}[b]{0.49\textwidth}
\includegraphics[width=1\linewidth]{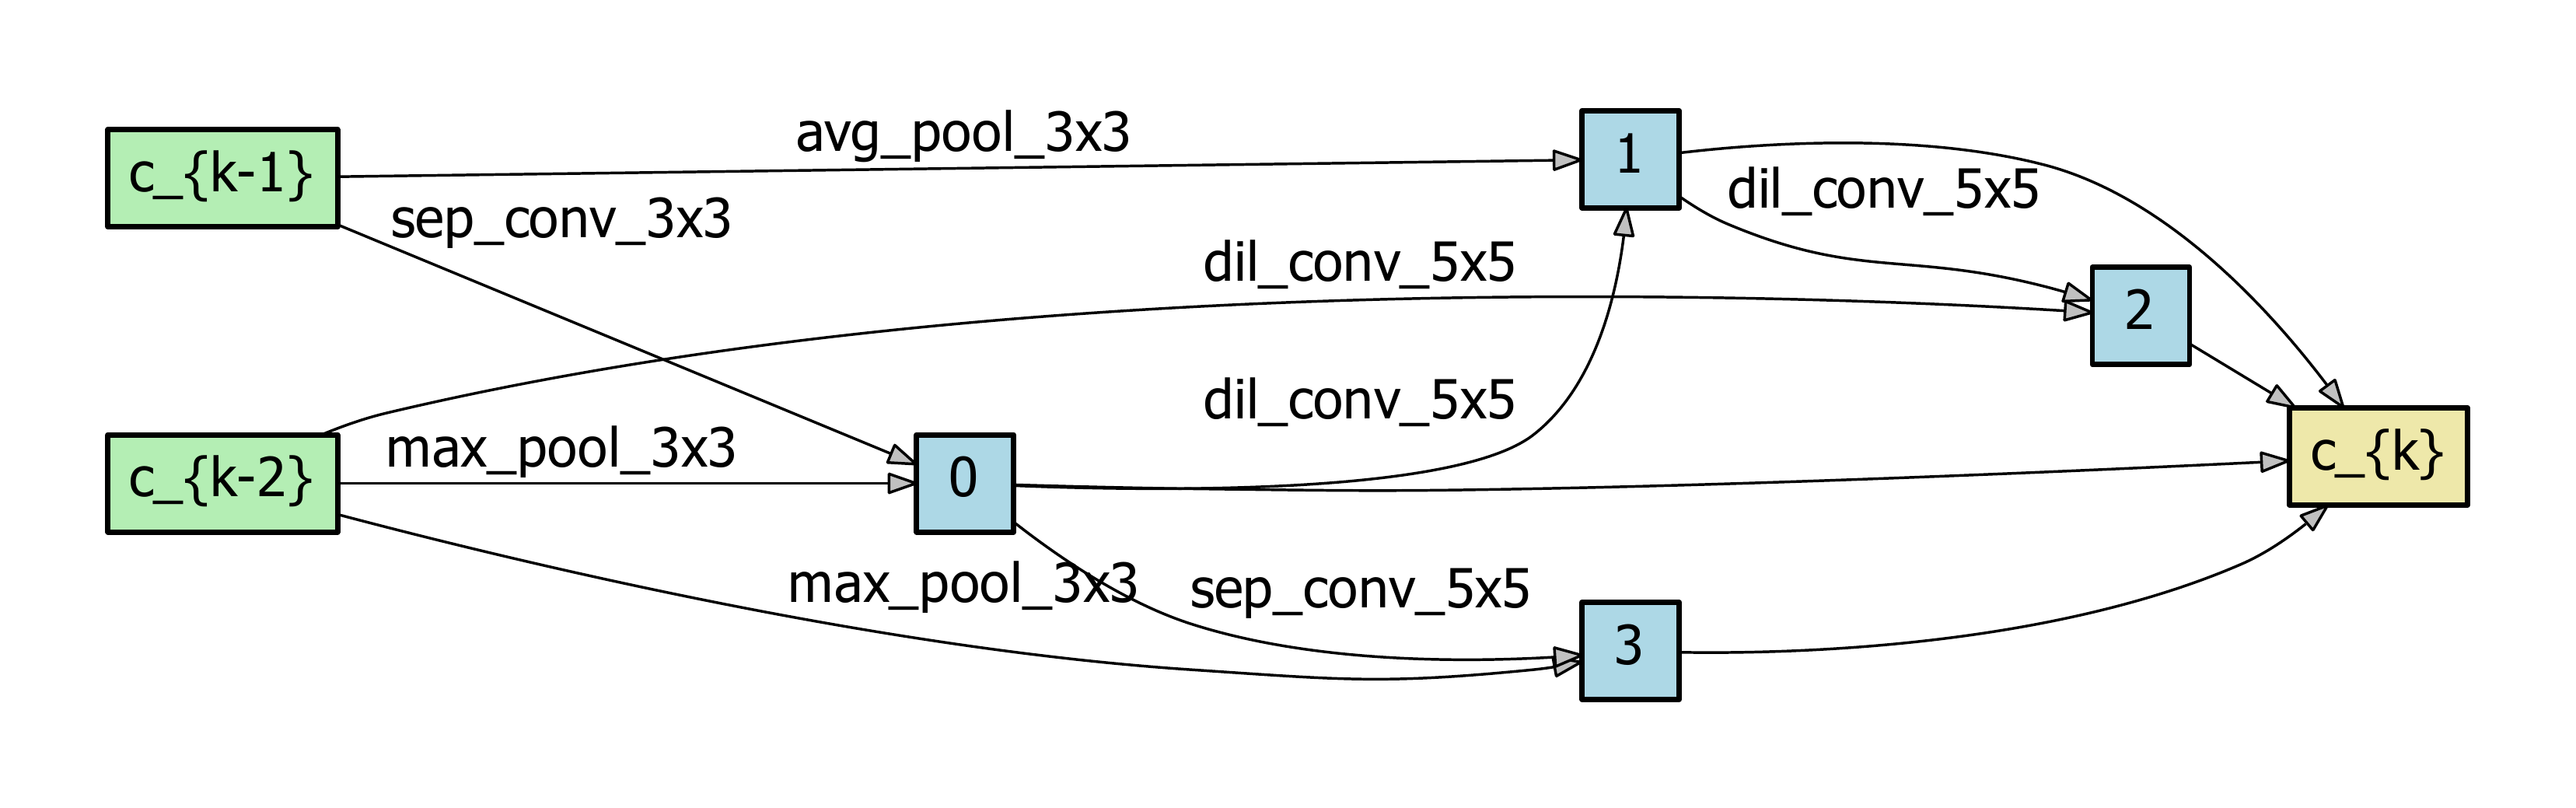}
        \caption{Reduction cell found on \textit{flower} task}
   \label{fig:Ng2}
    \end{subfigure}
    \caption{Abstract illustration of Neural Architecture Search methods \cite{elsken2019survey}.}
    \label{fig:search-space}
\end{figure}

\begin{figure}[]
    \centering
    \begin{subfigure}[b]{0.49\textwidth}
        \includegraphics[width=1\linewidth]{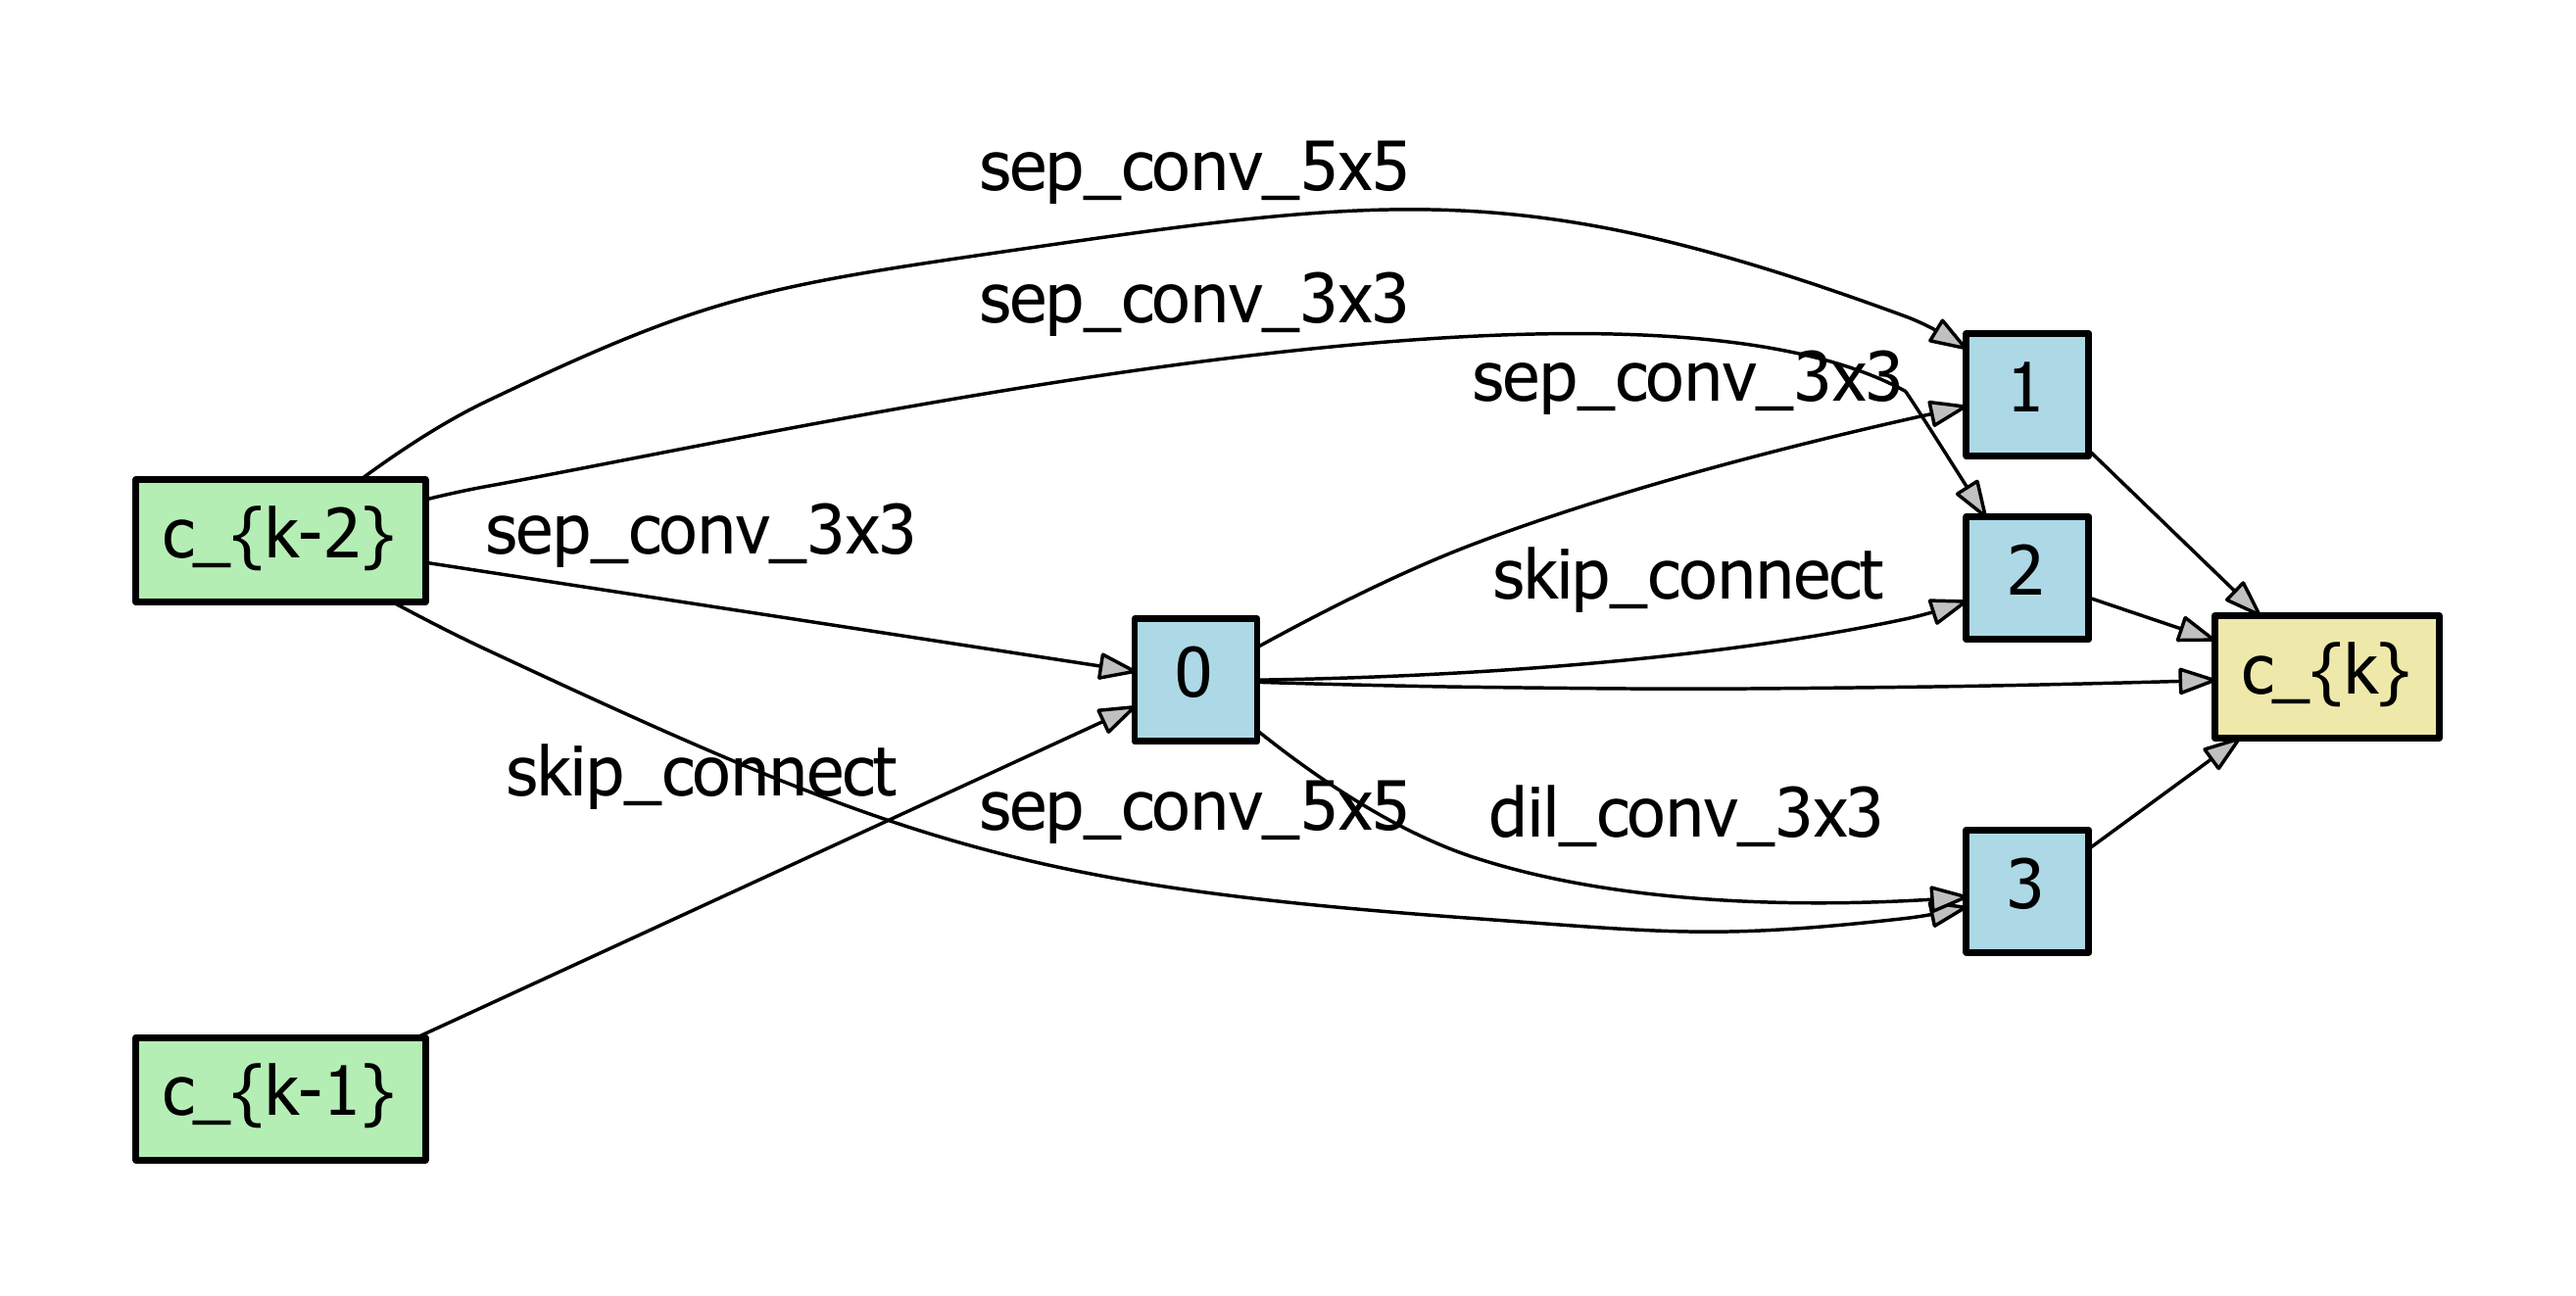}
        \caption{Normal cell found on \textit{flower} task}
   \label{fig:Ng1} 
    \end{subfigure}
    \begin{subfigure}[b]{0.49\textwidth}
\includegraphics[width=1\linewidth]{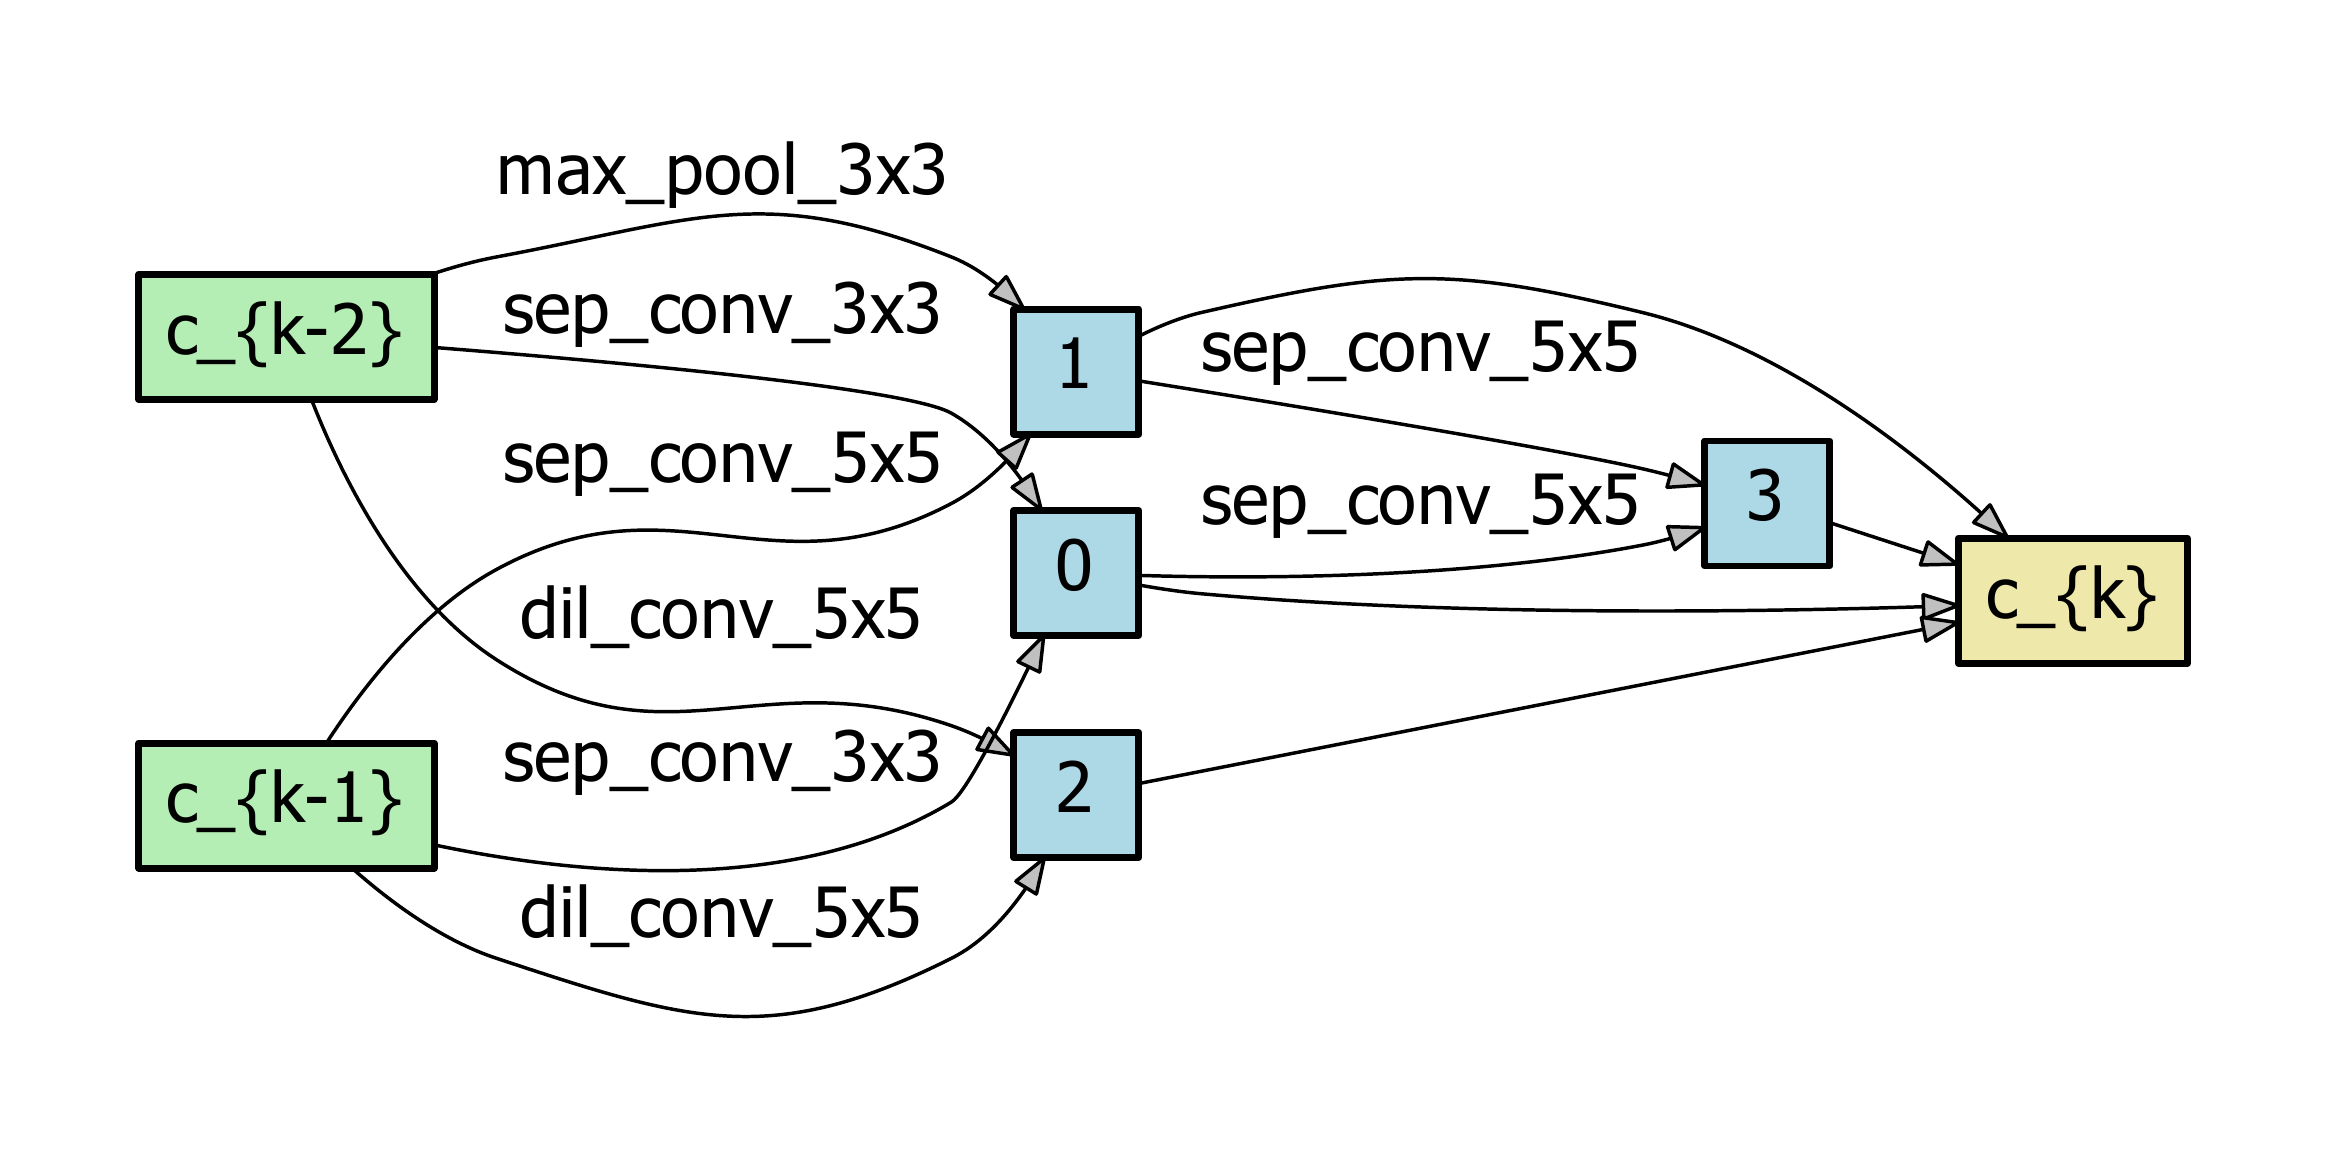}
        \caption{Reduction cell found on \textit{flower} task}
   \label{fig:Ng2}
    \end{subfigure}
    \begin{subfigure}[b]{0.49\textwidth}
        \includegraphics[width=1\linewidth]{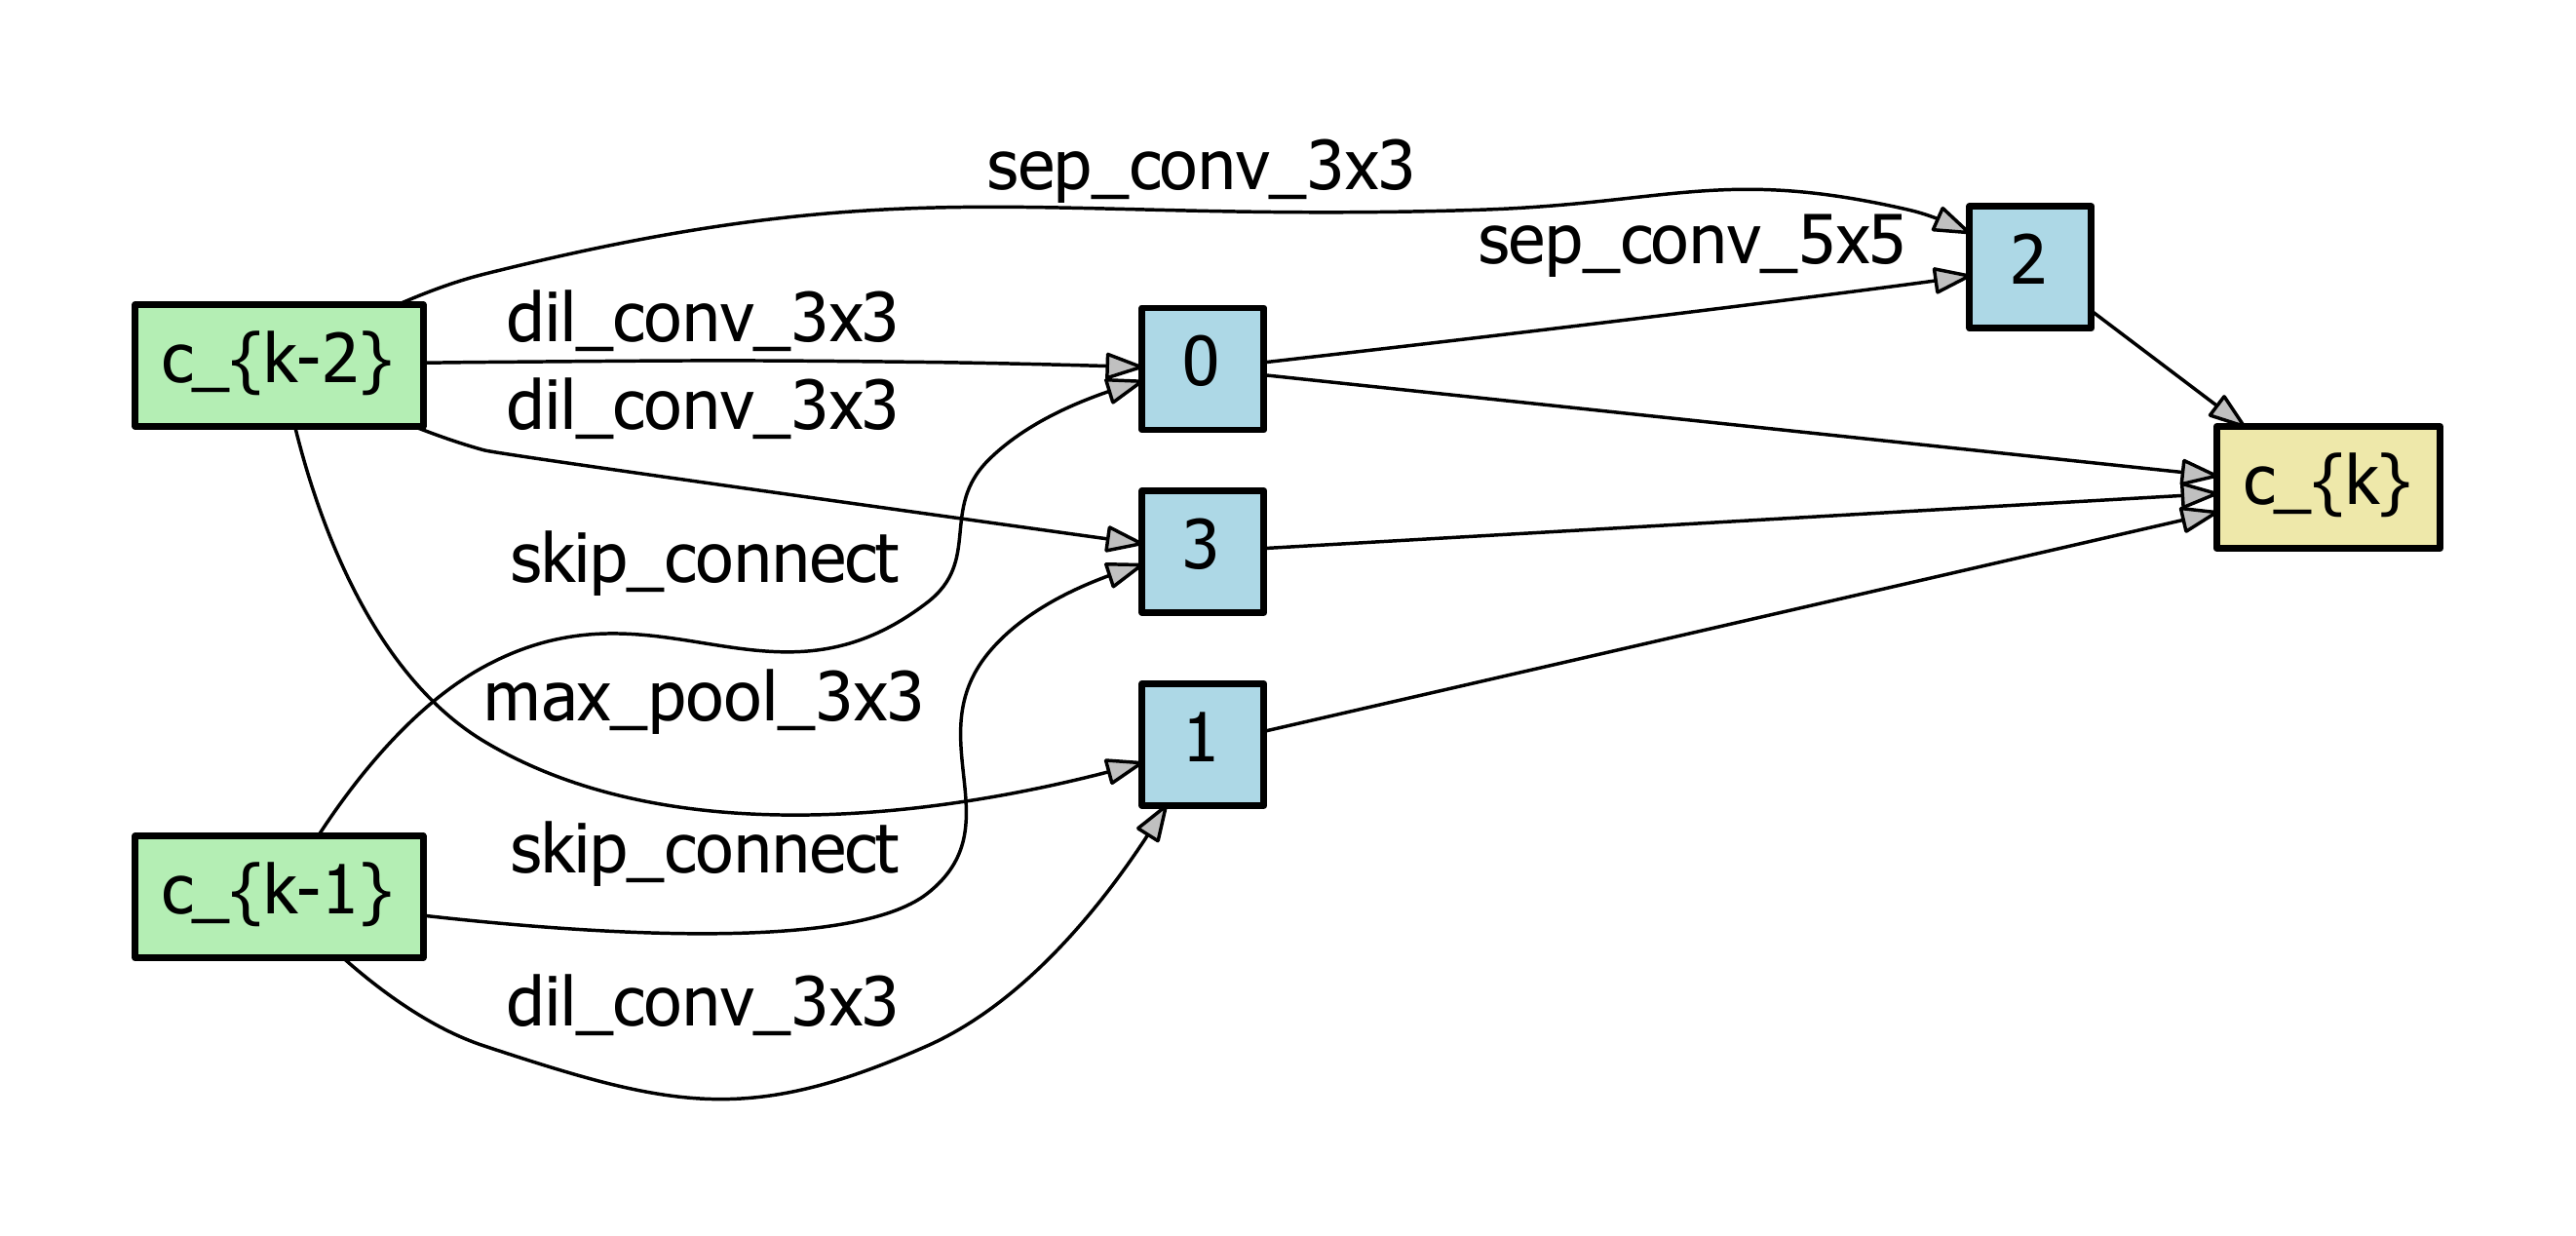}
        \caption{Normal cell found on \textit{flower} task}
   \label{fig:Ng1} 
    \end{subfigure}
    \begin{subfigure}[b]{0.49\textwidth}
\includegraphics[width=1\linewidth]{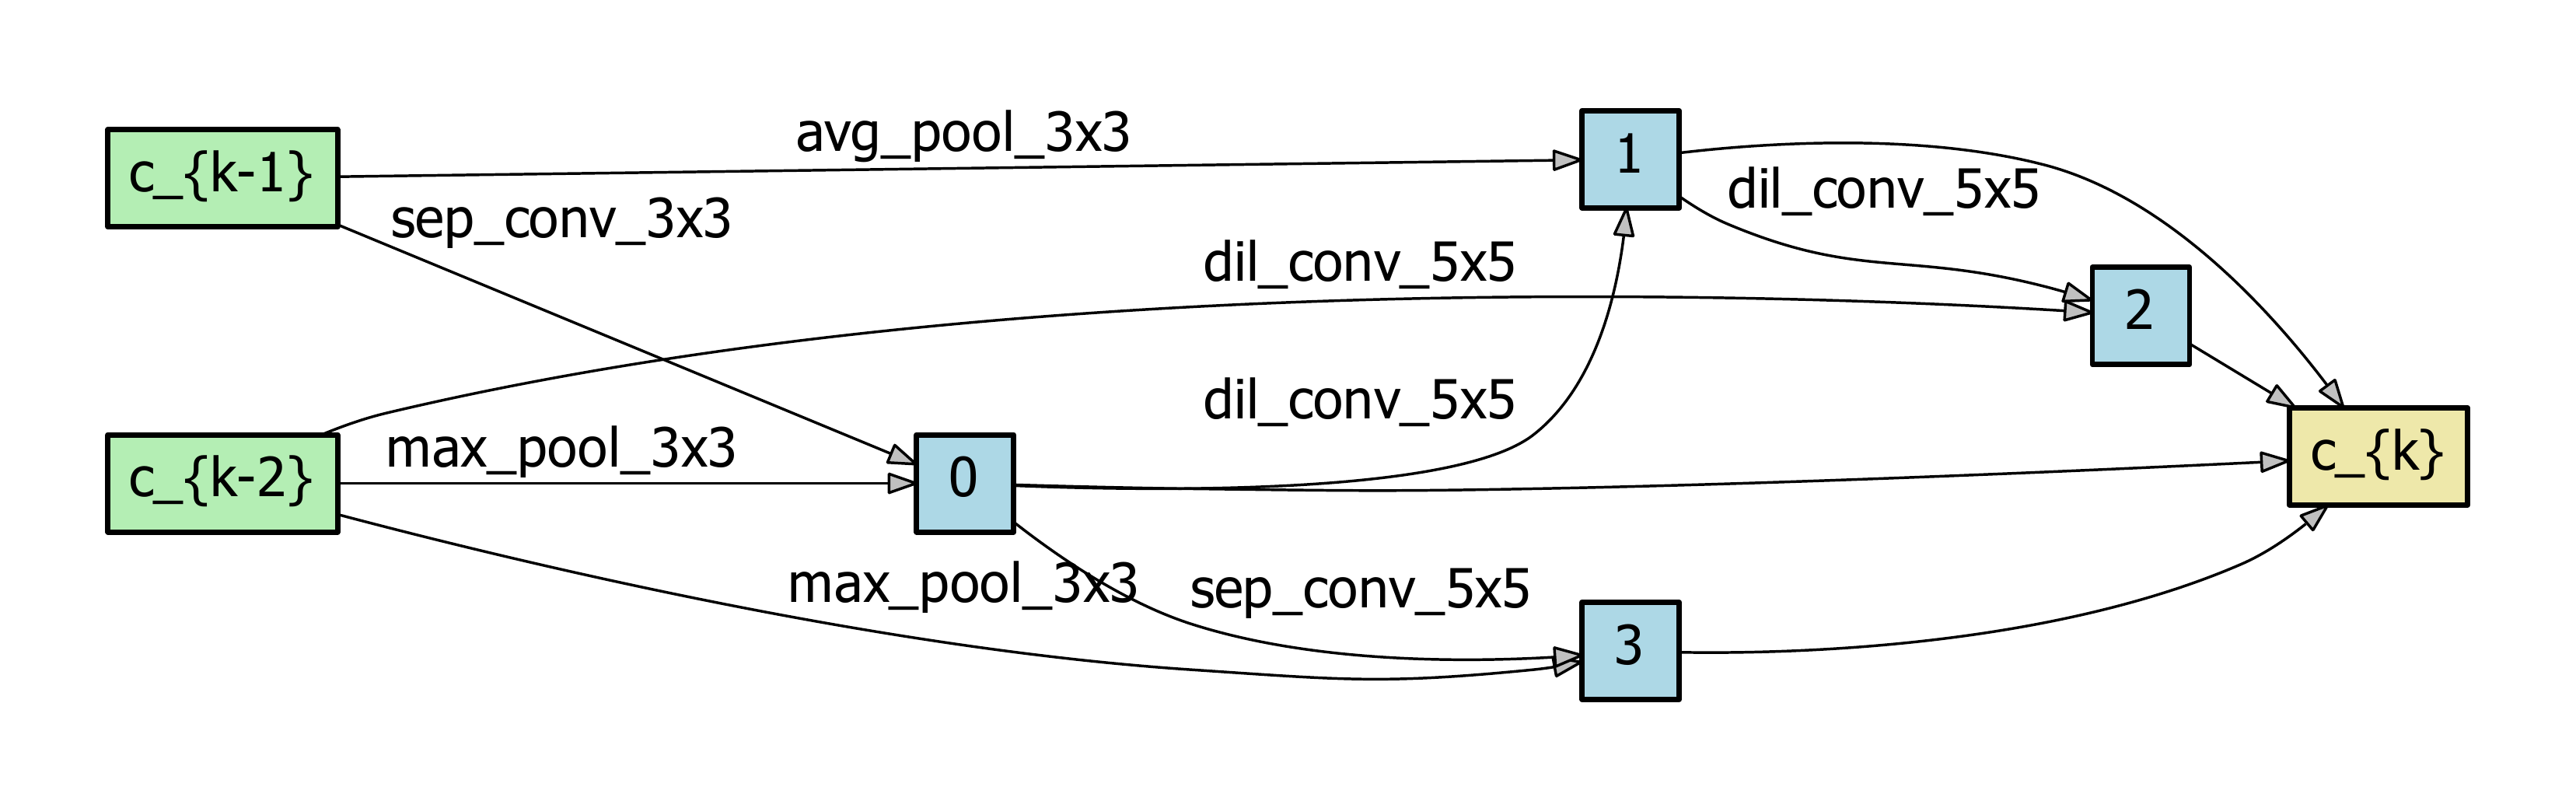}
        \caption{Reduction cell found on \textit{flower} task}
   \label{fig:Ng2}
    \end{subfigure}
    \caption{Abstract illustration of Neural Architecture Search methods \cite{elsken2019survey}.}
    \label{fig:search-space}
\end{figure}

\begin{figure}[]
    \centering
    \begin{subfigure}[b]{0.49\textwidth}
        \includegraphics[width=1\linewidth]{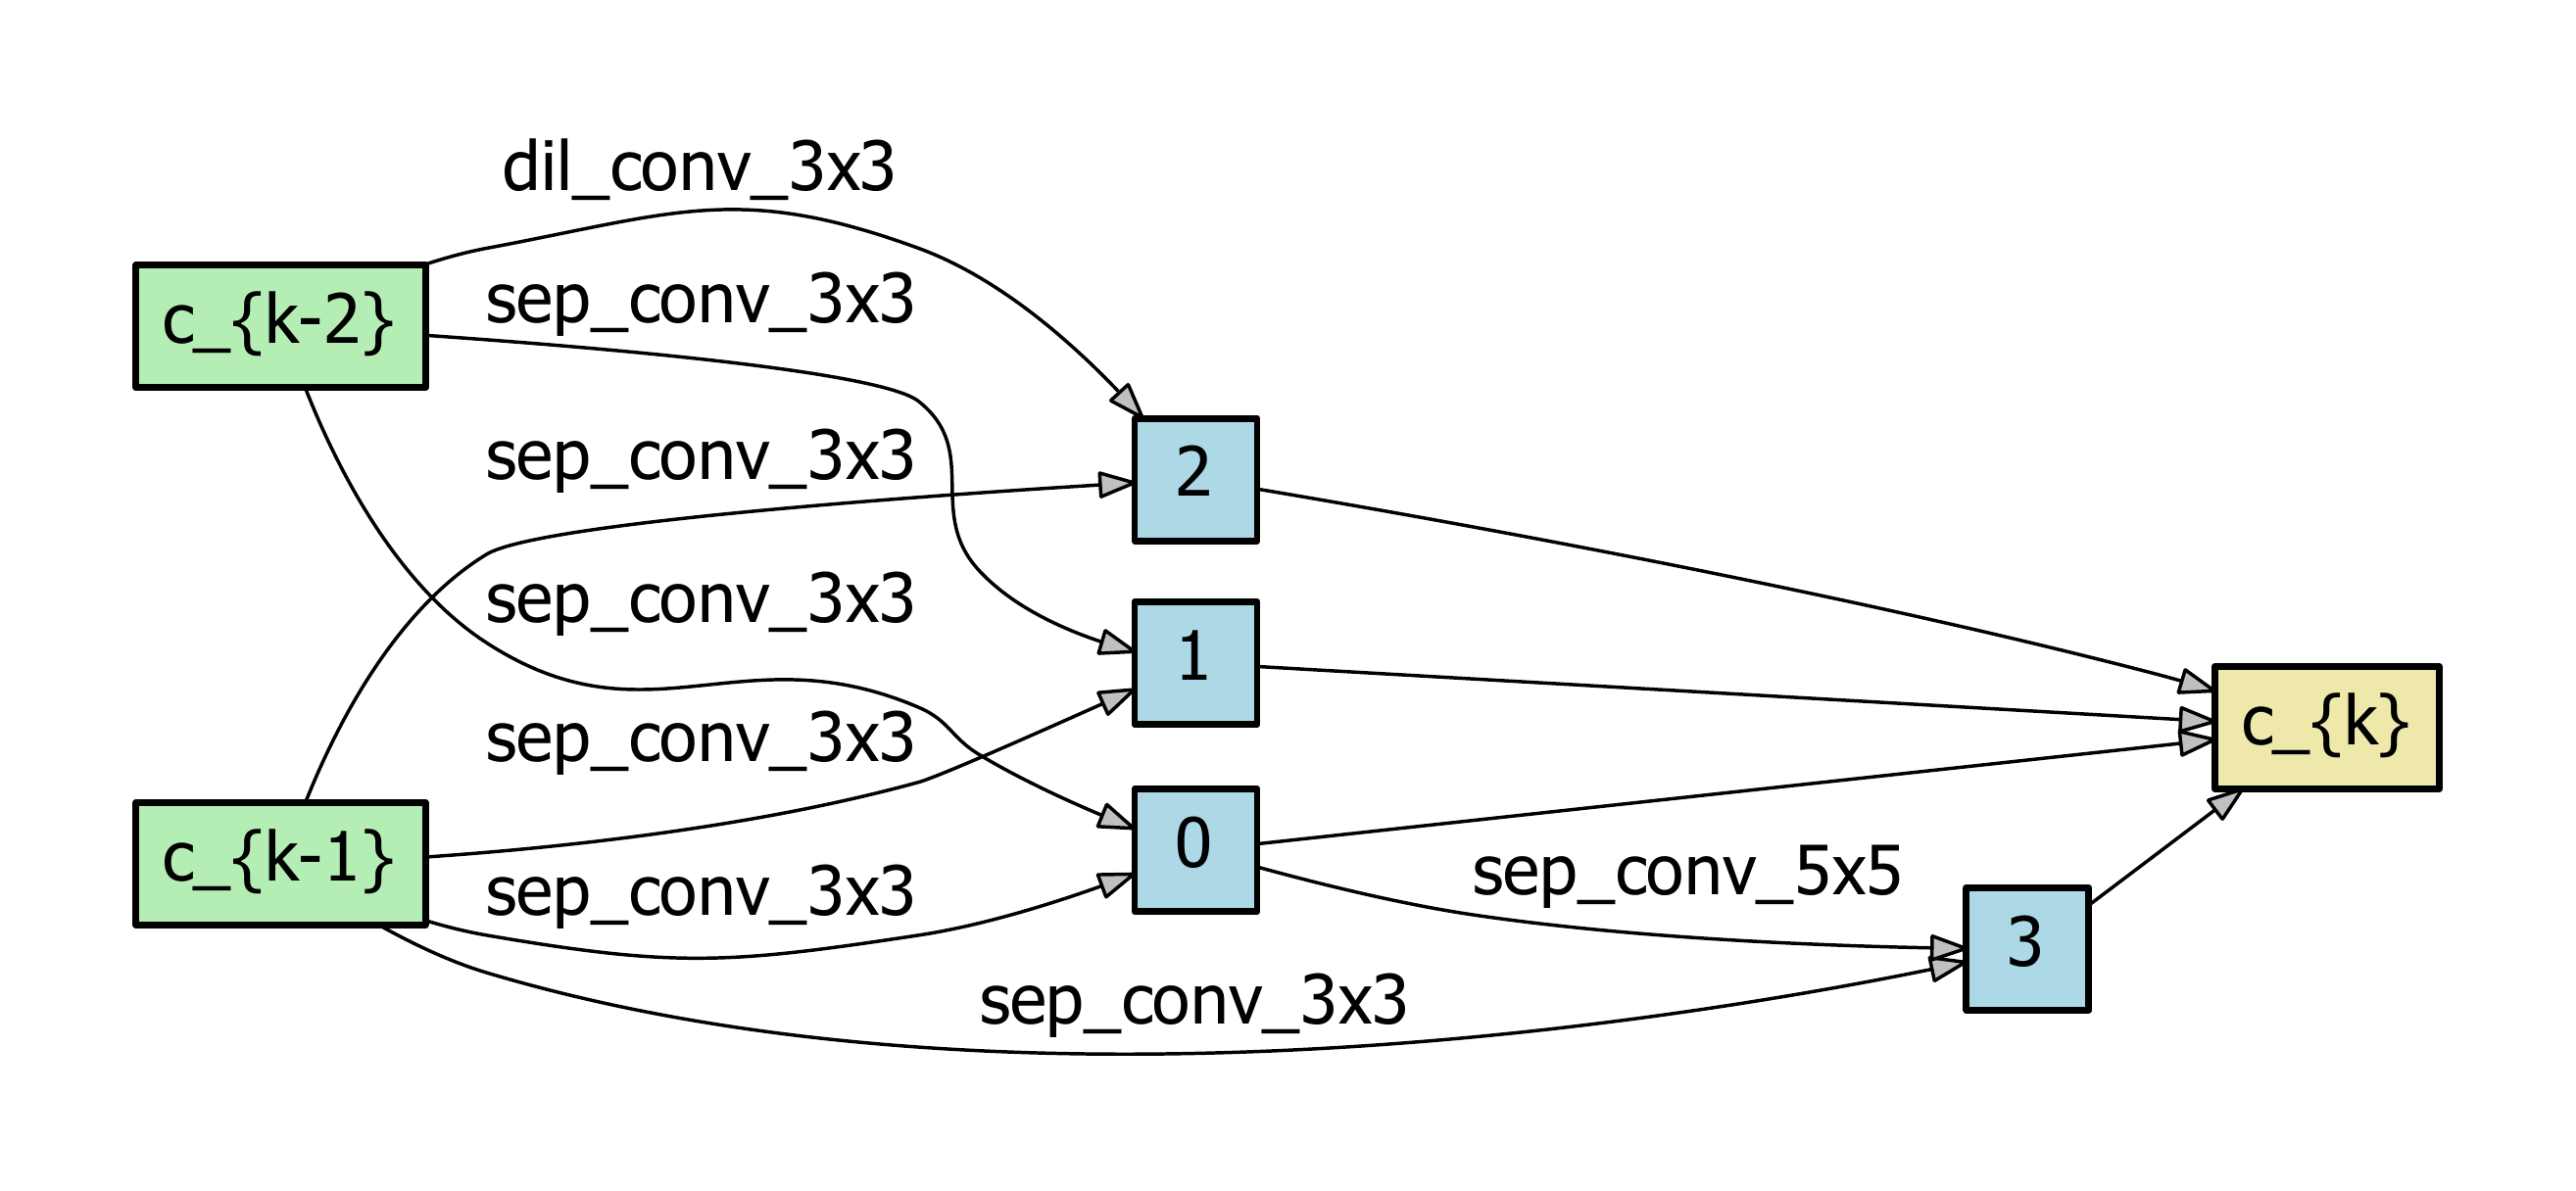}
        \caption{Normal cell found on \textit{flower} task}
   \label{fig:Ng1} 
    \end{subfigure}
    \begin{subfigure}[b]{0.49\textwidth}
\includegraphics[width=1\linewidth]{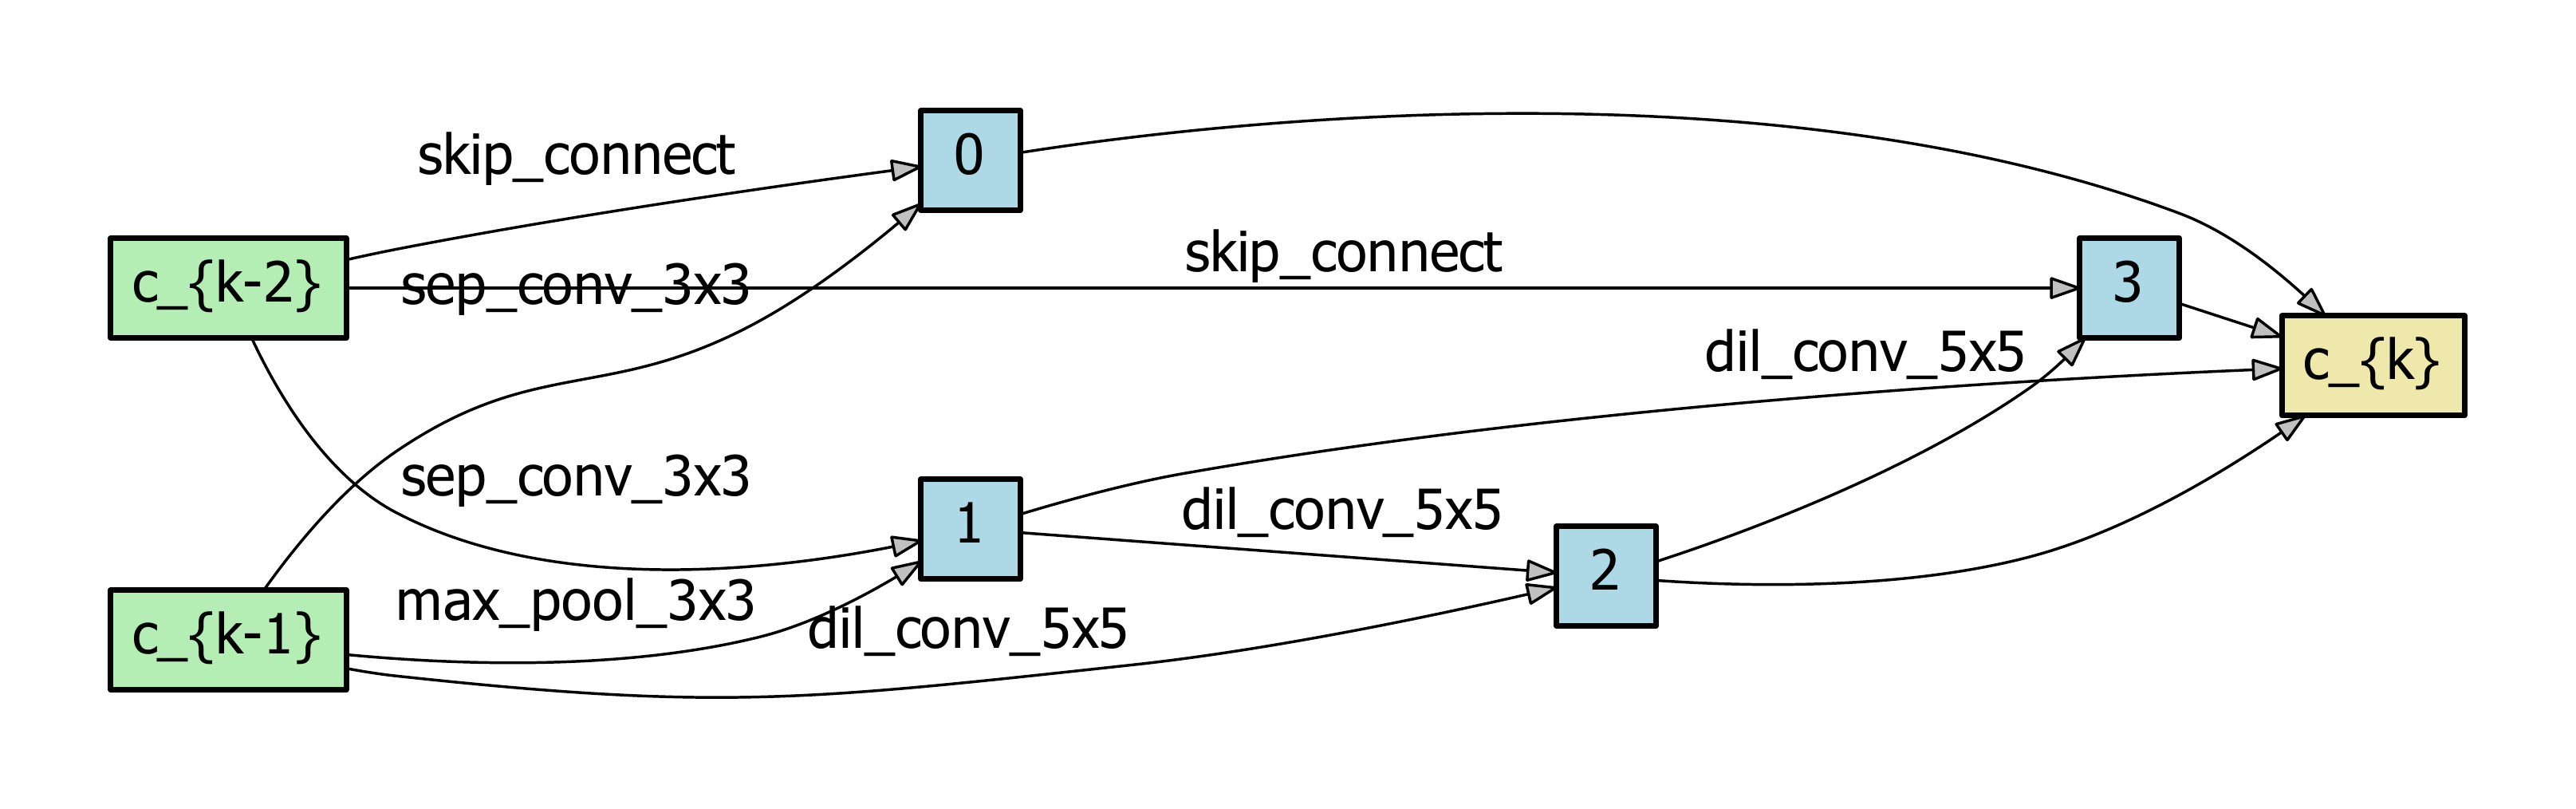}
        \caption{Reduction cell found on \textit{flower} task}
   \label{fig:Ng2}
    \end{subfigure}
    \begin{subfigure}[b]{0.49\textwidth}
        \includegraphics[width=1\linewidth]{cell/IN}
        \caption{Normal cell found on \textit{flower} task}
   \label{fig:Ng1} 
    \end{subfigure}
    \begin{subfigure}[b]{0.49\textwidth}
\includegraphics[width=1\linewidth]{cell/WWS_DTD_00v2-reduction-.pdf}
        \caption{Reduction cell found on \textit{flower} task}
   \label{fig:Ng2}
    \end{subfigure}
    \caption{Abstract illustration of Neural Architecture Search methods \cite{elsken2019survey}.}
    \label{fig:search-space}
\end{figure}

\begin{figure}[!h]
    \centering
    \begin{subfigure}[b]{0.49\textwidth}
    \centering
        \includegraphics[width=0.6\linewidth]{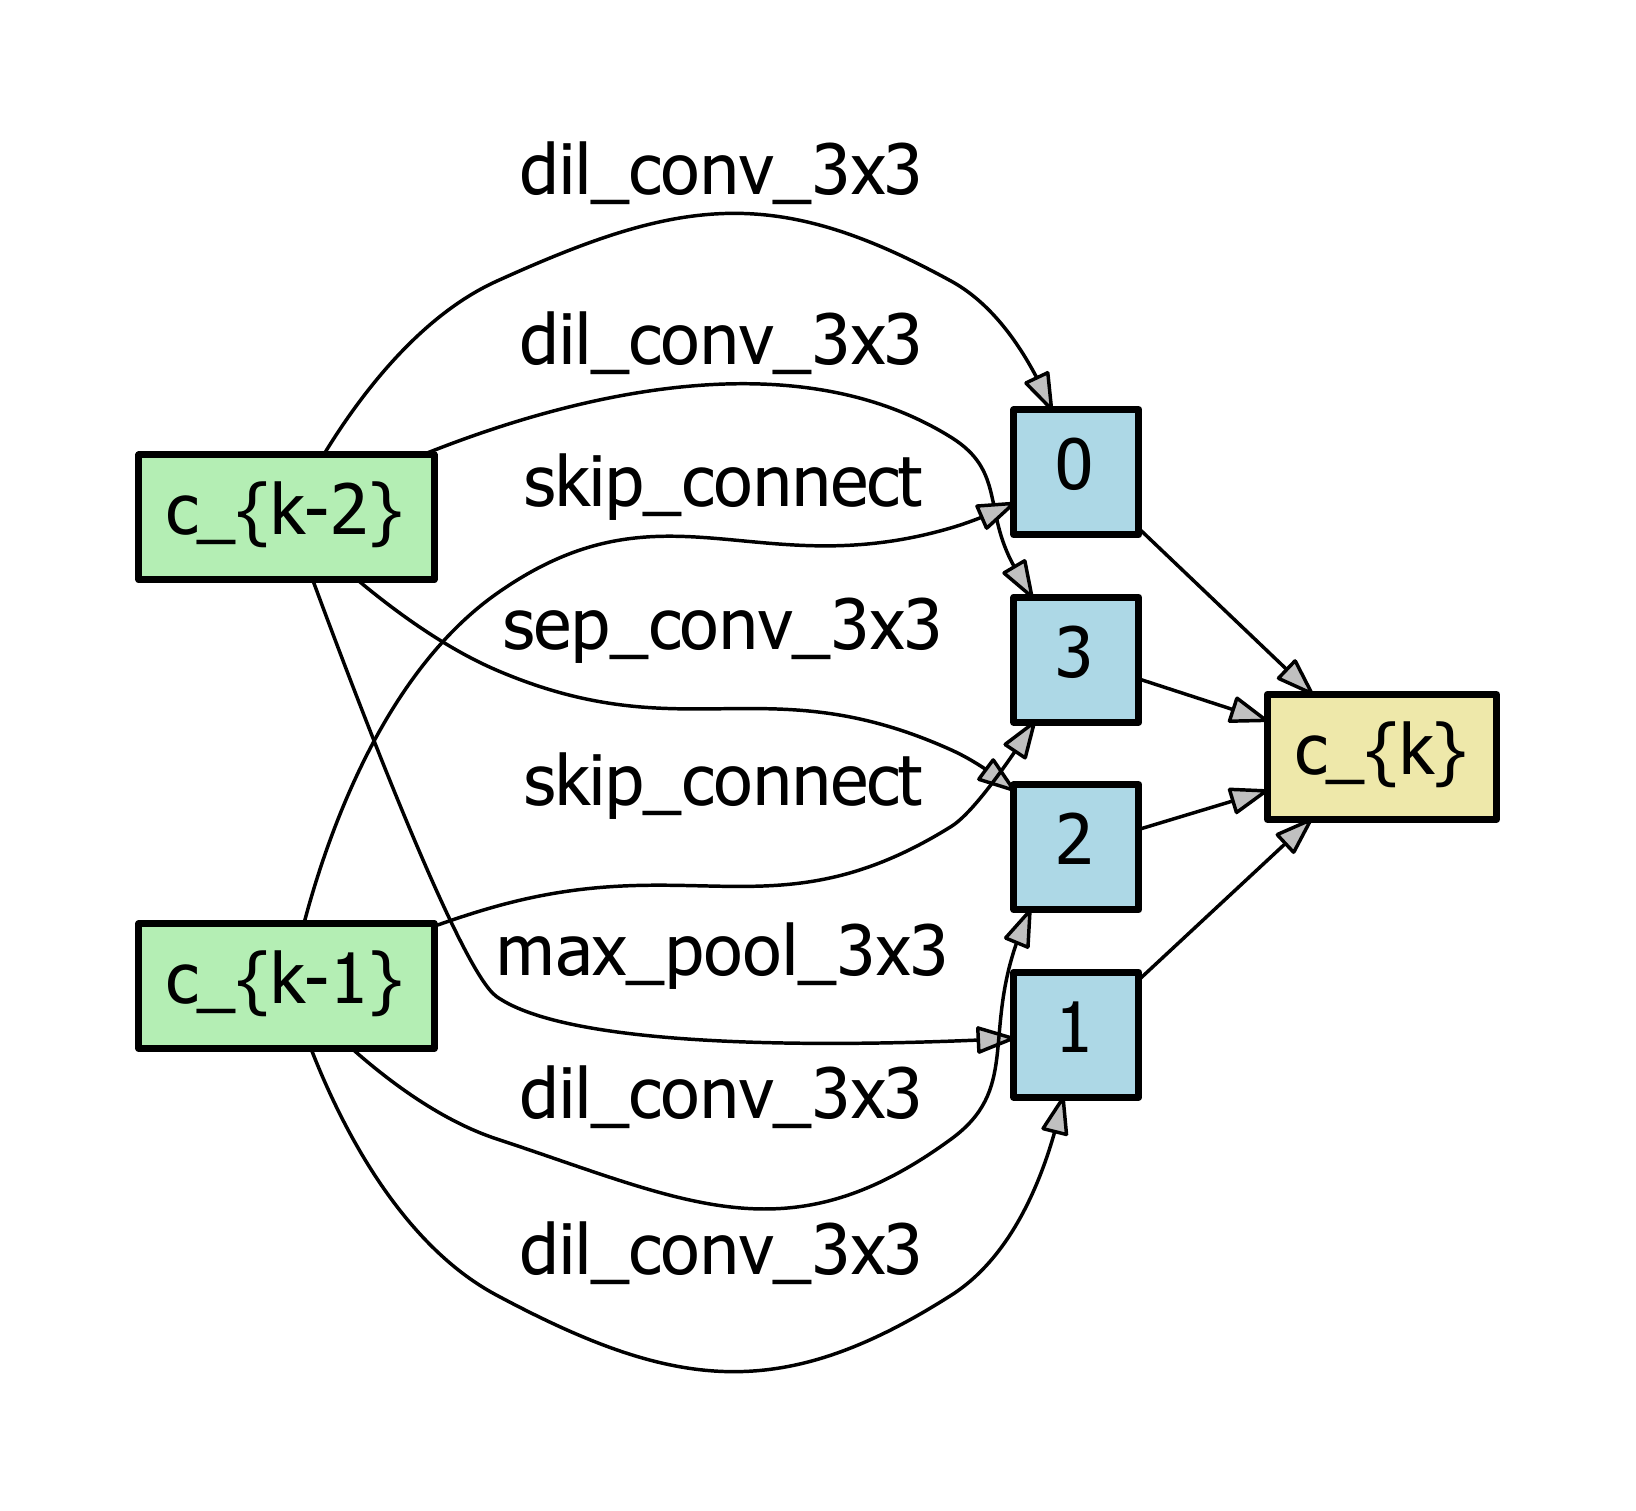}
        \caption{Normal cell found on \textit{tiny\_imagenet} task by P-DARTS algorithm.}
   \label{fig:Ng1} 
    \end{subfigure}
    \begin{subfigure}[b]{0.49\textwidth}
    \centering
        \includegraphics[width=1\linewidth]{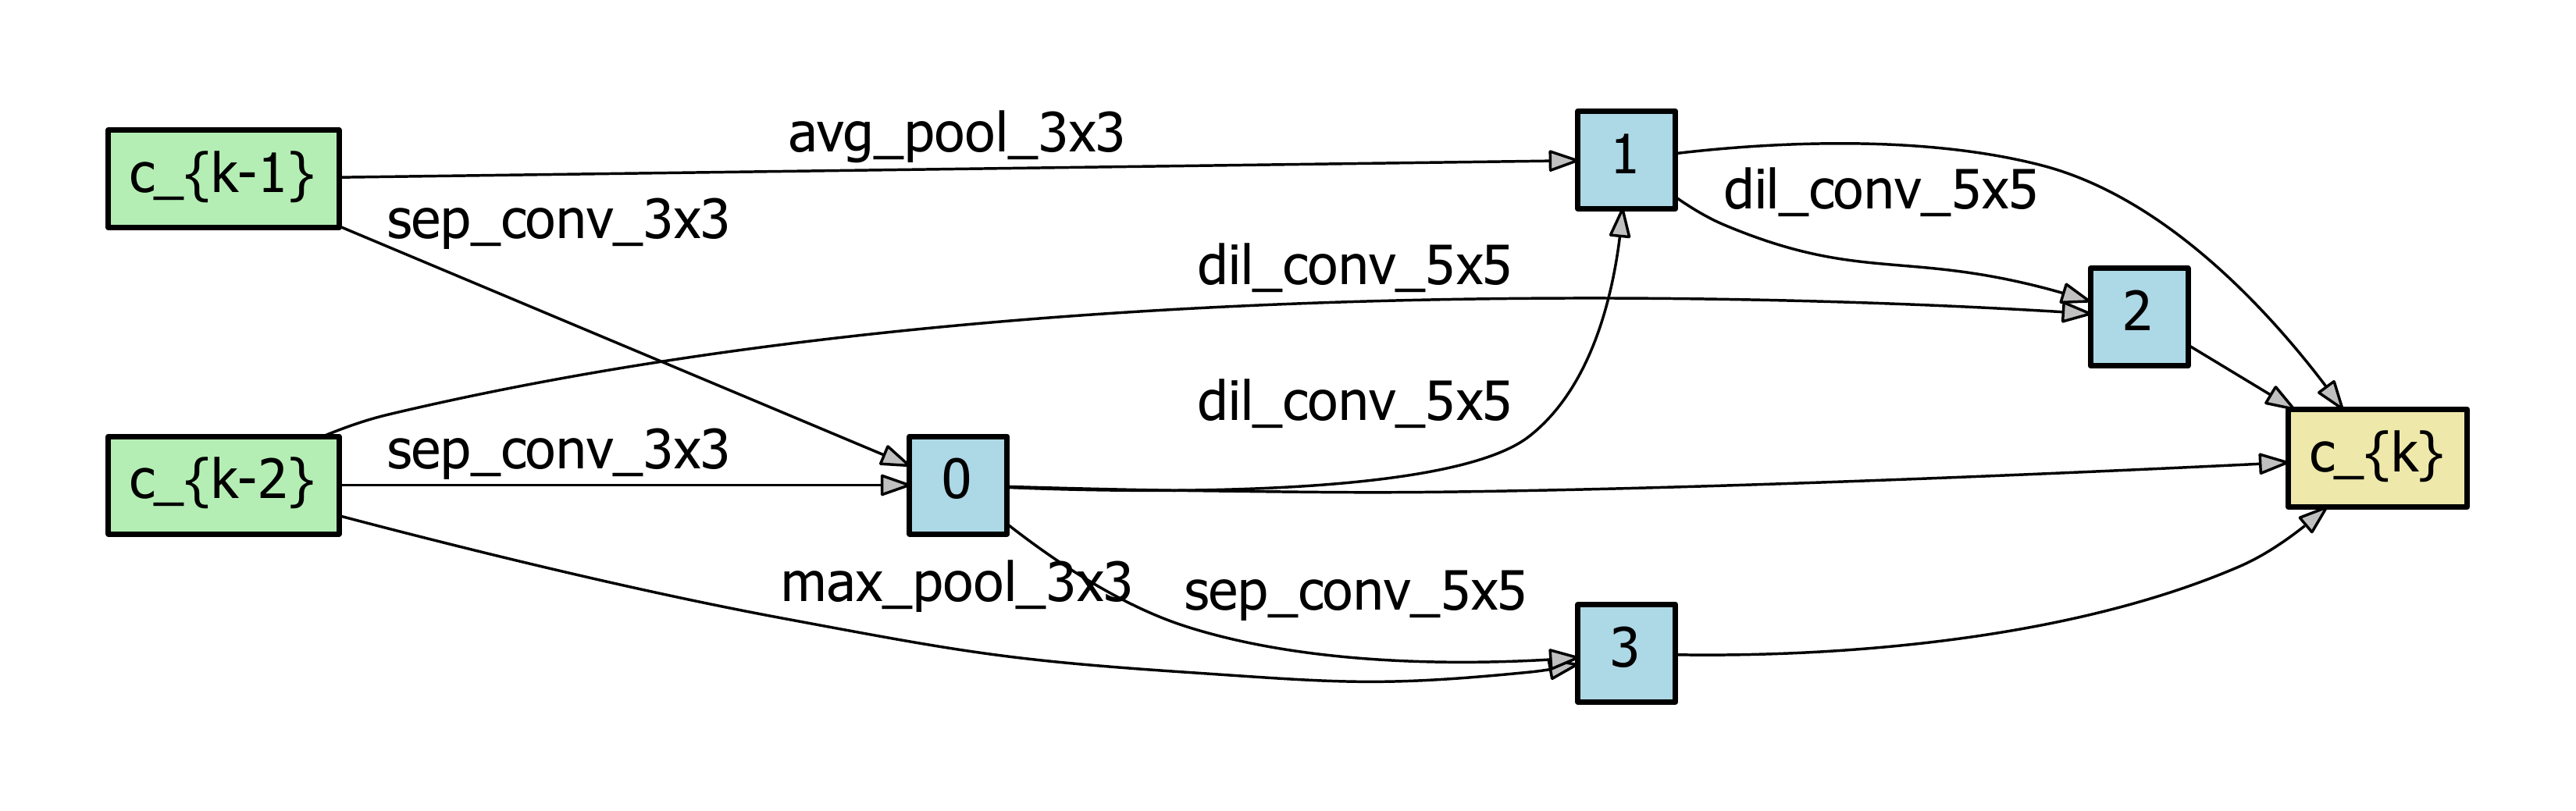}
        \caption{Reduction cell found on \textit{tiny\_imagenet} task by P-DARTS algorithm.}
   \label{fig:Ng2}
    \end{subfigure}
    \begin{subfigure}[b]{0.49\textwidth}
        \includegraphics[width=1\linewidth]{cell/WWS_DTD_00v2-normal.pdf}
        \caption{Normal cell found on \textit{dtd} task by WS-DARTS($\hat{\theta}_\text{tiny\_imagenet}$).}
   \label{fig:Ng1} 
    \end{subfigure}
    \begin{subfigure}[b]{0.49\textwidth}
\includegraphics[width=1\linewidth]{cell/WWS_DTD_00v2-reduction-.pdf}
        \caption{Reduction cell found on \textit{dtd} task by WS-DARTS($\hat{\theta}_\text{tiny\_imagenet}$).}
   \label{fig:Ng2}
    \end{subfigure}
    \caption{Comparison between cells discovered on \textit{tiny\_imagenet} from scratch using P-DARTS and cells discovered by WS-DARTS($\hat{\theta}_\text{tiny\_imagenet}$). }
    \label{fig:dtd}
\end{figure}
